# Supplementary material for: Chiral active hexatics: Giant number fluctuations, waves and destruction of order
Source: arXiv:2004.09115 ancillary file (2020-12-28)
Supplement: Supplementary file 1 [file chi_hex_abs.pdf]

# Chiral active hexatics: Giant number fluctuations, waves and destruction of order

Ananyo Maitra,<sup>1,\*</sup> Martin Lenz,<sup>2,3</sup> and Raphael Voituriez<sup>1,4</sup>

<sup>1</sup>*Sorbonne Université and CNRS, Laboratoire Jean Perrin, F-75005, Paris, France*

<sup>2</sup>*LPTMS, CNRS, Univ. Paris-Sud, Université Paris-Saclay, 91405 Orsay, France*

<sup>3</sup>*PMMH, CNRS, ESPCI Paris, PSL University, Sorbonne Université, Université de Paris, F-75005, Paris, France*

<sup>4</sup>*Sorbonne Université and CNRS, Laboratoire de Physique Théorique de la Matière Condensée, F-75005, Paris, France*

In this supplement we detail the calculations for the results discussed in the main text. The supplement is divided in two main sections: the first, Sec. I concerns the hexatic phase and the second, Sec. II the solid phase. Within Sec. I, in Sec. IA we discuss the equations of motion of chiral active hexatics and describe how the chiral active terms can be obtained from a description in which an auxiliary chemical coordinate is driven at a constant rate and in Sec. IB we obtain the phenomenological equations of motion of the active hexatic, in terms of the full order parameter, from detailed symmetry considerations. In Sec. IC we discuss the linear theory of a non-rotating chiral active hexatic, in Sec. ID we examine the linear theory of a rotating hexatic and in Sec. IE, fluctuations in a hexatic suspended in a momentum-conserved fluid. We then consider the dynamics of defects in the hexatic. In Sec. IF we discuss the dynamics of a single disclination, in Sec. IG we demonstrate that the far-field angle field due to a hexatic defect is modified due to activity, in Sec. IH we discuss the interactions between two hexatic defects and in Sec. II outline a theory of a hexatic with a finite density of disclinations. Finally, in Sec. IJ we discuss the implications of the results in the chiral hexatic phase for less symmetric chiral nematics. In the section on active chiral solids, Sec. II, we first consider chiral active solids on substrates Sec. IIA and then construct a phenomenological theory of dislocation unbinding and demonstrate that this yields the hydrodynamic equations for a chiral hexatic, in Sec. IIB.

## I. CHIRAL ACTIVE HEXATICS

### A. Active hexatics: Equations of motion

In this section we will present the equations of motion for active chiral hexatics which do not spontaneously rotate. Such phases have six-fold orientational symmetry but they lack any translational order. The local deviation from perfect hexatic order is characterised by the orientation field  $\theta(\mathbf{x}, t)$  while the local density of particles is characterised by  $\rho(\mathbf{x}, t)$ . The local velocity field of the active hexatic is characterised by the velocity field  $\mathbf{v}(\mathbf{x}, t)$ . The conserved dynamics of the density field is given by the continuity equation

$$\partial_t \rho = -\nabla \cdot (\rho \mathbf{v}). \quad (\text{I.A.1})$$

The general dynamical equation for the angle field is

$$\frac{d}{dt} \theta = \frac{1}{2} \epsilon_{ij} \partial_i v_j + \gamma_c \nabla \cdot \mathbf{v} - \Gamma_6 \frac{\delta F}{\delta \theta} + \xi_\theta = \frac{1}{2} \epsilon_{ij} \partial_i v_j + \gamma_c \nabla \cdot \mathbf{v} + \Gamma_6 K \nabla^2 \theta + \xi_\theta \quad (\text{I.A.2})$$

where  $d/dt \equiv \partial_t + \mathbf{v} \cdot \nabla$ ,  $F$  is the free energy, which for hexatics is simply  $F = \int d\mathbf{r} K (\nabla \theta)^2 / 2 + f(\rho)$ , where  $f(\rho)$  is a function of density and

$$\epsilon = \begin{pmatrix} 0 & 1 \\ -1 & 0 \end{pmatrix} \quad (\text{I.A.3})$$

is the levi-civita tensor. The first term on the R.H.S. of (I.A.2) denotes the precession of the angle field in a local vorticity field [25]. The second term is more complicated and is only present in chiral systems with  $\gamma_c$  being a chiral coefficient whose sign depends on the chirality of the particles. In a chiral hexatic the angle field can precess due to a local isotropic compressional or dilational velocity field with the direction of precession depending on chirality. Note that while this term is chiral, it is *not necessarily* active and can be present in passive chiral hexatics as well. The third term controls the relaxation of the bond-angle order parameter to its equilibrium value in the absence of activity and flow with  $\Gamma_6$  being a dissipative kinetic coefficient. Finally,  $\xi_\theta$  is a Gaussian white noise with strength  $\Delta_\theta$ .

Finally, the equation for the velocity field is

$$\rho \frac{d}{dt} \mathbf{v} = -\gamma_c K \nabla \nabla^2 \theta - \frac{K}{2} (\hat{z} \times \nabla) \nabla^2 \theta - K \nabla \theta \nabla^2 \theta - \rho \nabla \frac{\delta F}{\delta \rho} - \zeta \hat{z} \times \nabla \theta - \zeta_c \hat{z} \times (\hat{z} \times \nabla) \theta - \Gamma \mathbf{v} + \Gamma_c \hat{z} \times \mathbf{v} + \xi_v \quad (\text{I.A.4})$$

The first term on the the R.H.S. in (I.A.4) denotes an equilibrium chiral force conjugate to  $\gamma_c \nabla \cdot \mathbf{v}$  in (I.A.2) as required by Onsager symmetry in the absence of activity. This term (as well as  $\gamma_c \nabla \cdot \mathbf{v}$  on the R.H.S. of (I.A.2)) is not present in theories of equilibrium achiral hexatics, but it doesn't change either the steady-state distribution or the equal-time correlation functions implying that the steady-state of equilibrium chiral and achiral hexatics are equivalent. The reason for this is that it is a reversible coupling which does not affect the steady-state distribution. We can check this directly by examining the Rayleigh dissipation functional

$$\mathcal{R} = \int \partial_t \mathbf{g} \cdot \frac{\delta \mathcal{H}}{\delta \mathbf{g}} + \partial_t \theta \frac{\delta \mathcal{H}}{\delta \theta} \quad (\text{I.A.5})$$

where  $\mathbf{g} = \rho \mathbf{v}$ , the phenomenological Hamiltonian  $\mathcal{H} = F + \int g^2/2\rho$  and  $\delta \mathcal{H}/\delta \mathbf{g} = \mathbf{v}$ . To show that the terms with the coefficient  $\gamma_c$  do not contribute to  $\mathcal{R}$ , we simply replace  $\partial_t \mathbf{g}$  by  $\gamma_c \nabla \delta \mathcal{H}/\delta \theta$  and  $\partial_t \theta$  by  $\gamma_c \nabla \cdot \delta \mathcal{H}/\delta \mathbf{g}$  which yields

$$\int \gamma_c \frac{\delta \mathcal{H}}{\delta \mathbf{g}} \cdot \nabla \frac{\delta \mathcal{H}}{\delta \theta} + \int \gamma_c \frac{\delta \mathcal{H}}{\delta \theta} \nabla \cdot \frac{\delta \mathcal{H}}{\delta \mathbf{g}} = 0 \quad (\text{I.A.6})$$

by integration by parts. The second term in (I.A.4) is an equilibrium force present in achiral passive hexatics that is the counterpart of the  $(1/2)\epsilon_{ij}\partial_i v_j$  term in (I.A.2). The third term is an Onsager counterpart of the advective nonlinearity in (I.A.2) and is ignored in the main text since it only leads to irrelevant nonlinear terms once the velocity field is integrated out. The fourth term is the usual passive density coupling that ultimately yields the pressure (note that this term involves  $F$  and *not*  $\mathcal{H}$  – the term appearing from the kinetic part of the phenomenological Hamiltonian in the reversible density-momentum coupling cancels a term appearing from the reversible momentum-momentum coupling to yield the usual advective nonlinearity and this term). The fifth term  $\propto \hat{z} \times \nabla \theta$  is an achiral but active force. This force implies an explicitly antisymmetric stress and therefore can only be present in systems in which angular momentum is not conserved [4]. The sixth term on the R.H.S. of (I.A.4), which can be written as  $\zeta_c \nabla \theta$ , is another active force. Note that since  $\theta$  itself is a pseudoscalar variable, this term is explicitly chiral, with the handedness being encoded in the sign of  $\zeta_c$ . The seventh term encodes the friction of the hexatic fluid with the substrate. The eighth term is an *active chiral* friction. It has the same form as a Lorentz force on a charged particle in a plane in the presence of a magnetic field perpendicular to the plane. It is not present in passive systems on substrate (which conserves neither momentum nor angular momentum) since *any* dissipative coupling in passive systems, in the absence of magnetic fields, has to be symmetric [3] and this coupling is explicitly anti-symmetric. The final term is a Gaussian spatiotemporally white noise with strength  $\Delta_v$ . Thus, the hexatic is driven out of equilibrium due to the action of *three* terms with coefficients  $\Gamma_c$ ,  $\zeta$  and  $\zeta_c$ . In the absence of these terms, i.e.  $\Gamma_c = \zeta_c = \zeta = 0$ , if the noise strengths  $\Delta_\theta = 2T\Gamma_6$  and  $\Delta_v = 2T\Gamma$ , these equations describe an *equilibrium* hexatic whose steady state distribution is  $\propto e^{-\mathcal{H}/T}$  (since  $\mathcal{H}$  doesn't contain any chiral term, the equilibrium steady-state distribution is the same for both chiral and achiral hexatics, as discussed out earlier). This can be checked by writing down the functional Fokker-Planck equation corresponding to (I.A.1), (I.A.2) and (I.A.4) and solving for a state with no *dissipative* current. However, the steady-state distribution *will* be modified due to the active terms and the steady-state will, in general, feature dissipative configuration currents.<sup>1</sup>

The existence of the active terms can be *formally* argued for by using the formalism discussed in [23]. There we formally introduced a chemical coordinate  $n$  and its conjugate momentum  $m$ , extended the free energy to  $\tilde{F} = F + \int f_n(n) + m^2/2$  and wrote down the coupled dynamics of all fields. Carrying out this programme here, and declaring that  $n$  (which is even under time-reversal) only couples to the momentum density, we obtain

$$\partial_t \mathbf{g} = -\mathcal{C}_{\mathbf{g}m} \frac{\delta \tilde{F}}{\delta m} + T \frac{\delta \mathcal{C}_{\mathbf{g}m}}{\delta m} - \Gamma \frac{\delta \tilde{F}}{\delta \mathbf{g}} - \Gamma_{\mathbf{g}m} \frac{\delta \tilde{F}}{\delta m} \dots \quad (\text{I.A.7})$$

where the ellipsis denotes the reactive couplings between the density and the angle fields and the momentum density fields, and a white noise of strength.  $\mathcal{C}_{\mathbf{g}n}$  is the Poisson bracket between  $\mathbf{g}$  and  $n$  which can depend on *all* fields, and which may, in principle, be calculated from a microscopic theory which would incorporate the couplings between chemical and mechanical degrees of freedom. We will not do that here, and instead will only write down a form of  $\mathcal{C}_{\mathbf{g}n}$  that is allowed by symmetry. The second term on the R.H.S., with  $T$  being the temperature, is required for obtaining the correct steady-state distribution (required by detailed balance) [14], but luckily is 0 in most cases, including the one we will be dealing with (see [23] for examples of cases in which it is non-zero). The equation of motion for  $n$  is simply  $\partial_t n = \delta \tilde{F}/\delta m = m$  and the one for  $m$  is taken to be

$$\partial_t m = -\mathcal{C}_{m\mathbf{g}} \cdot \frac{\delta \tilde{F}}{\delta \mathbf{g}} + T \frac{\delta}{\delta \mathbf{g}} \cdot \mathcal{C}_{m\mathbf{g}} - \frac{\delta \tilde{F}}{\delta n} - \Gamma_n^{-1} \frac{\delta \tilde{F}}{\delta m} - \Gamma_{m\mathbf{g}} \cdot \frac{\delta \tilde{F}}{\delta \mathbf{g}} + \xi_n \quad (\text{I.A.8})$$

<sup>1</sup> We have neglected active contributions due to density variations. These can be both achiral  $\propto \nabla \rho$  and chiral  $\propto \hat{z} \times \nabla \rho$ .

where the noise  $\xi_n$  has the correlation. The noise strengths are chosen to be proportional to the dissipative coefficients with a proportionality factor  $T$ . This dynamics obeys detailed balance by construction. Now, we define  $\mathcal{C}_{\mathbf{g}m} = \{\mathbf{g}(\mathbf{x}), m(\mathbf{x}')\} = -\boldsymbol{\epsilon} \cdot \mathbf{v}(\mathbf{x})\delta(\mathbf{x} - \mathbf{x}') = -\mathcal{C}_{m\mathbf{g}}$ , take

$$\Gamma_{m\mathbf{g}} = \tilde{\zeta}\boldsymbol{\epsilon} \cdot \nabla\theta + \tilde{\zeta}_c\nabla\theta \quad (\text{I.A.9})$$

and take the overdamped limit in (I.A.8) to replace

$$m = \partial_t n = -\Gamma_n \frac{\delta\tilde{F}}{\delta n} - \Gamma_n \Gamma_{m\mathbf{g}} \cdot \mathbf{v} + \Gamma_n \xi_n. \quad (\text{I.A.10})$$

When we replace the  $m$  in

$$\partial_t \mathbf{g} = \boldsymbol{\epsilon} \cdot \mathbf{v} m - \Gamma \mathbf{v} - (\tilde{\zeta}\boldsymbol{\epsilon} \cdot \nabla\theta + \tilde{\zeta}_c\nabla\theta)m... \quad (\text{I.A.11})$$

by the R.H.S. of (I.A.10) and *crucially, imposing a drive on the chemical cocordinate* by taking  $\langle \delta\tilde{F}/\delta n \rangle = \text{const.} = \Delta\mu$ , which *makes the model active*, we now get, to the lowest order in fields,

$$\partial_t \mathbf{g} = -\Gamma_n \Delta\mu \boldsymbol{\epsilon} \cdot \mathbf{v} - \Gamma \mathbf{v} + \Gamma_n \Delta\mu (\tilde{\zeta}\boldsymbol{\epsilon} \cdot \nabla\theta + \tilde{\zeta}_c\nabla\theta)... \quad (\text{I.A.12})$$

This yields the active terms in (I.A.4) with  $\Gamma_c = \Gamma_n \Delta\mu$ ,  $\zeta = \Gamma_n \Delta\mu \tilde{\zeta}$  and  $\zeta_c = \Gamma_n \Delta\mu \tilde{\zeta}_c$ .

### B. Equations of motion for the bond-angle order parameter and density: Detailed symmetry-based arguments

In this section, we write down the general coupled phenomenological equations of motion for the bond-angle order parameter and the density field, without reference to an auxiliary velocity field, purely based on symmetry. The definition of the bond-angle order parameter, as earlier, is

$$\Psi = \psi e^{6i\theta}; \quad \Psi^* = \psi e^{-6i\theta} \quad (\text{I.B.1})$$

and we have also defined its complex conjugate. The conserved density field is denoted by the scalar  $\rho$ . The current in the density equation,  $\mathbf{J} = J_x \hat{x} + J_y \hat{y}$  can be written as

$$J = J_x + iJ_y; \quad J^* = J_x - iJ_y. \quad (\text{I.B.2})$$

with the conservation law

$$\partial_t \rho = \frac{1}{2}(\nabla^* J + \nabla J^*) \quad (\text{I.B.3})$$

where

$$\nabla = \partial_x + i\partial_y; \quad \nabla^* = \partial_x - i\partial_y. \quad (\text{I.B.4})$$

The hydrodynamic equations would consist of all terms that are allowed by symmetry. In an achiral system, these symmetries would be

- Rigid rotation of space and spin: Rotate the coordinate frame and the spins by the same angle.
- Reflection for achiral systems: Reflection along any plane perpendicular to the plane. In particular, the  $y - z$  and the  $x - z$  plane
- Independent rotation of with space or spin through  $\pi/3$

Under a rigid rotation through an arbitrary angle  $\delta\theta$ ,

$$\theta \rightarrow \theta - \delta\theta \implies \Psi \rightarrow \Psi e^{-i6\delta\theta}; \quad \Psi^* \rightarrow \Psi^* e^{i6\delta\theta} \quad (\text{I.B.5})$$

$$\nabla \rightarrow e^{-i\delta\theta} \nabla; \quad \nabla^* \rightarrow e^{i\delta\theta} \nabla^* \quad (\text{I.B.6})$$

$$J \rightarrow e^{-i\delta\theta} J; \quad J^* \rightarrow e^{i\delta\theta} J^* \quad (\text{I.B.7})$$

Similarly, under reflection through  $y - z$  plane:

$$x \rightarrow -x; \quad y \rightarrow y; \quad \theta \rightarrow \pi - \theta \quad (\text{I.B.8})$$

$$\Psi \rightarrow \Psi_0 e^{i6(\pi-\theta)} = \Psi^*, \quad \Psi^* \rightarrow \Psi \quad (\text{I.B.9})$$

$$\nabla \rightarrow -\partial_x + i\partial_y = -\nabla^*; \quad \nabla^* \rightarrow -\nabla \quad (\text{I.B.10})$$

$$J \rightarrow -J^*; \quad J^* \rightarrow -J \quad (\text{I.B.11})$$

and under reflection through  $x - z$  plane

$$x \rightarrow x; \quad y \rightarrow -y; \quad \theta \rightarrow -\theta \quad (\text{I.B.12})$$

$$\Psi \rightarrow \Psi^*; \quad \Psi^* \rightarrow \Psi \quad (\text{I.B.13})$$

$$\nabla \rightarrow \nabla^*; \quad \nabla^* \rightarrow \nabla \quad (\text{I.B.14})$$

$$J \rightarrow J^*; \quad J^* \rightarrow J \quad (\text{I.B.15})$$

Chiral systems are symmetric under rotation but, crucially, *not* under reflection. Any vector transforms under rotation as  $A \rightarrow e^{-i\delta\theta} A$  and under reflection through  $y - z$  as  $A \rightarrow -A^*$  and through  $x - z$  as  $A \rightarrow A^*$ . In the real space, one can construct a vector that is not symmetric under reflections, from a vector  $\mathbf{A} = (A_x, A_y)$  that is:  $\mathbf{A}_c = \epsilon \cdot \mathbf{A} = (A_y, -A_x)$ . For the complex vectors this implies  $A_c = -i(A_x + iA_y) = A_y - iA_x$ . With this information we can now construct the equations of motion. First, the current in the density equation must transform under rotation as a vector and therefore, must be of the form

$$J = s_1 \nabla(\Psi\Psi^*) + s_2 \Psi^* \nabla \Psi + s_3 \nabla \rho + s_{c1} i \nabla(\Psi\Psi^*) + s_{c2} i \Psi^* \nabla \Psi + s_{c3} i \nabla \rho + \dots \quad (\text{I.B.16})$$

where the terms with coefficients  $s_i$  are symmetric under reflection and thus allowed in all active hexatic systems while those with coefficient  $s_{ci}$  are not and therefore only allowed in chiral hexatic systems. Higher order terms in fields and gradients can be constructed by noting that all such terms must have the same rotational symmetries of those in (I.B.16) and thus, can be obtained from them by operating on them with the pair of operators  $\nabla$  and  $\nabla^*$  or multiplication by  $\Psi$  and  $\Psi^*$  or by  $\rho$ . The first term which cannot be obtained this way is  $\nabla^* \Psi$ . To construct the dynamical equation for  $\partial_t \Psi$ , we note that under rotation,  $\partial_t \Psi \rightarrow e^{-i6\delta\theta} \partial_t \Psi$ . Therefore, it's equation of motion must have the form

$$\partial_t \Psi = a_1 \Psi + a_2 \nabla \nabla^* \Psi + a_3 \Psi \nabla \nabla^* \rho + a_4 \Psi \nabla \nabla^* (\Psi\Psi^*) + a_{c1} i \Psi + a_{c2} i \nabla \nabla^* \Psi + a_{c3} i \Psi \nabla \nabla^* \rho + a_{c4} i \Psi \nabla \nabla^* (\Psi\Psi^*) + \dots \quad (\text{I.B.17})$$

where the terms with coefficient  $a_i$  are achiral and those with coefficients  $a_{ci}$  are chiral.

Eq. (I.B.16) and (I.B.17) have a *higher* symmetry than the ones under which they were derived. They are symmetric under *independent* rotations of *space* or *spin* by an *arbitrary* angle. To see this, note that the equations are symmetric under  $\Psi \rightarrow \Psi e^{-i6\delta\theta}$  *without* transforming  $J$  or  $\nabla$  and under  $J \rightarrow J e^{-i\delta\theta}$  and  $\nabla \rightarrow e^{-i\delta\theta} \nabla$  *without* transforming  $\Psi$ . This is a spurious symmetry which exists because of the order in gradients to which we have expanded our equations. The lowest order in gradient terms that would break this symmetry in a hexatic (I.B.16) are  $\nabla^* \nabla^* \nabla^* \nabla^* \nabla^* \Psi$  and  $i \nabla^* \nabla^* \nabla^* \nabla^* \nabla^* \Psi$ , while the lowest order linear term in (I.B.17) is  $\nabla^6 \rho$ . In a triatic, terms that break this spurious symmetry appear with *two* gradients in the triatic version of (I.B.16), while in a tetratic, such terms arise at third order in gradients. In a nematic, they appear at *first* order in gradients in (I.B.16) and they are  $\nabla^* \Psi_2$  (achiral) and  $i \nabla^* \Psi_2$  (chiral) where  $\Psi_2 = \psi e^{2i\theta}$  is the nematic order parameter. The  $\nabla^* \Psi_2$  current in achiral nematics, when expressed in terms of the angle field deep in the ordered phase leads to a term  $\propto \partial_x \partial_y \theta$  in the  $\partial_t \rho$  equation and is responsible for *giant number fluctuations* in *achiral* nematics. However, giant number fluctuations *require chirality* in triatics or tetratics or hexatics.

Since *both* (I.B.16) and (I.B.17) possess an extra symmetry under *independent* rotations of space and spin by arbitrary angles at this order in gradients, they *also* describe an active and chiral variant of XY model coupled to an

auxiliary conserved field (not a chiral version of Vicsek model which explicitly breaks the symmetry under independent rotations of space and spin and strictly speaking, should be described as an active variant of a model of chiral polar liquid crystal, whose spatial symmetries it shares and not an active variant of an XY model which has a higher spatial symmetry). Therefore, these equations should also describe the dynamics of driven dissipative condensates coupled to an extra conserved field [18, 35]. The Malthusian version (i.e., one in which the density is *not* a conserved quantity, but is held *locally* fixed) of our model for a chiral, active hexatic was indeed considered in these contexts [18, 35].

From (I.B.16) and (I.B.17), we can now obtain the coupled density, bond angle equations from these by considering the imaginary part of the  $\Psi$  equation and the  $\rho$  equation and taking  $\psi = \text{const.}$  deep in the hexatic phase. The linear coupled equations are

$$\partial_t \rho = s_3 \nabla^2 \rho - 6s_{c2} \psi^2 \nabla^2 \theta \quad (\text{I.B.18})$$

$$\partial_t \theta = \frac{a_{c1}}{6} + a_2 \nabla^2 \theta + \frac{a_{c3}}{6} \nabla^2 \rho \quad (\text{I.B.19})$$

where  $\nabla^2 = (\partial_x^2 + \partial_y^2)$ . Thus, we again discover that there is no linear coupling between  $\rho$  and  $\theta$  in an achiral hexatic but there is in chiral hexatics. Here, the term with the coefficient  $a_{c1}$  leads to spontaneous rotation of the ordered phase. The first achiral linear coupling between density and the angle field arises at sixth order in gradients from the current term  $\nabla^* \Psi$  in the density equation and the term  $\nabla^6 \rho$  in the equation from  $\Psi$ . As discussed, this reflects the hexagonal symmetry of the system.

We can also write down the full coupled equation for  $\Psi$ ,  $v = v_x + iv_y$  and  $\rho$  using this notation, which we now do for completeness. The density field obeys the equation

$$\partial_t \rho = \frac{1}{2} [\nabla(\rho v^*) + \nabla^*(\rho v)]. \quad (\text{I.B.20})$$

The hexatic order parameter obeys the equation

$$\partial_t \Psi + \frac{1}{2} [v \nabla^* + v^* \nabla] \Psi = i\Omega[\rho] \Psi + \frac{n\Psi}{4} [\nabla^* v - \nabla v^*] + \frac{in\gamma_c}{2} \Psi [\nabla^* v + \nabla v^*] - 2n^2 \Gamma_6 \frac{\delta F_\Psi}{\delta \Psi^*} \quad (\text{I.B.21})$$

where, for clarity, we have not displayed allowed Onsager couplings which do not contribute to the angle equation in the hexatic phase and  $n > 2$  is the symmetry of the ordered phase, with hexatics having  $n = 6$ . The existence of  $\Omega$  requires both activity and chirality and its consequences will be discussed in Sec. ID. The velocity field has the equation of motion

$$\begin{aligned} \rho \left[ \partial_t + \frac{1}{2} (v \nabla^* + v^* \nabla) \right] v = \frac{1}{2} \left[ (\nabla \Psi) \frac{\delta F_\Psi}{\delta \Psi} + (\nabla \Psi^*) \frac{\delta F_\Psi}{\delta \Psi^*} \right] + \left( \frac{n}{4} - \frac{in\gamma_c}{2} \right) \nabla \left[ \Psi^* \frac{\delta F_\Psi}{\delta \Psi^*} - \Psi \frac{\delta F_\Psi}{\delta \Psi} \right] \\ - \left[ \frac{\zeta}{n} + \frac{i\zeta_c}{n} \right] \Psi^* \nabla \Psi - \rho \nabla \frac{\delta F_\Psi}{\delta \rho} - (\Gamma - i\Gamma_c) v \end{aligned} \quad (\text{I.B.22})$$

which can be seen to reduce to (I.A.4) upon taking  $\Psi = \psi_0 e^{in\theta}$  with a constant  $\psi_0 = 1$  and writing the free energy as

$$F_\Psi = \int d\mathbf{x} f(\rho) + \int d\mathbf{x} \frac{K}{2n^2} \left[ |\nabla \Psi|^2 + \frac{1}{2\zeta^2} (1 - |\Psi|^2)^2 \right]. \quad (\text{I.B.23})$$

This set of equations are symmetric under *independent* rotations of space and spin variables. These are also the most general equations at this order in gradients when  $n > 2$  and reduce to (I.A.1), (I.A.2) and (I.A.4) when  $\psi_0$  assumes a constant value. However, for  $n = 1$  (polar) or  $n = 2$  a larger number of active and passive terms are allowed at this order in gradients by symmetry. Those terms break the symmetry under independent rotations of space and spin to one under joint rotations of *both*. Therefore, chiral active nematic and polar models are likely to have a distinct phase behaviour not captured by these equations of motion. Note that while the expression for the active forces  $\propto \Psi^* \nabla \Psi$  and  $\propto i\Psi^* \nabla \Psi$  can be written as  $\epsilon \cdot \nabla \theta$  and  $\nabla \theta$  when  $\psi_0$  is a constant, they cannot be written as a gradient of scalar or a divergence of a symmetric tensor otherwise. Therefore, these forces are not allowed in systems that conserve momentum.

Though the active forces written in terms of the angle field seem to be a divergence of a rank two tensor, the force on a physical boundary (with an active hexatic inside and nothing outside, i.e., across which the order parameter magnitude goes from a finite value to 0) is not the line integral of this tensor since the active forces written in terms of the full order parameter are not total divergences. Indeed, the force on a physical boundary is difficult to calculate, but

their form can be obtained from the following symmetry argument. In passive systems, the force on the boundary of a region, which contains a hexatic inside and an isotropic fluid outside, does not depend on the relative angle between the boundary and the hexatic field i.e. rotating the hexatic by a constant angle does not change the boundary force. However, boundary forces generically depend on the relative angle between the local normal to the surface and the orientation field at the boundary in active systems. In an active hexatic, the boundary forces at an interface with a distinguished normal, written as a complex number with a unit magnitude,  $N = N_x + iN_y = e^{i\phi}$ , are of the form  $N[N^6\Psi^* + (N^6\Psi^*)^*]$ ,  $N^{*5}\Psi$ ,  $iN[N^6\Psi^* + (N^6\Psi^*)^*]$  and  $iN^{*5}\Psi$  where the last two are chiral. The first of these is along the local normal (by construction) while the third, chiral one is purely tangential. All these forces explicitly depend on the relative angle between the normal and the direction of ordering at the boundary. Such boundary forces may, in principle, automatically emerge from the forces considered here in the presence of a surface separating a hexatic region from an isotropic region, for example.

### C. Linear theory of chiral active hexatic: Non-rotating state

In this section we will present the linearised hydrodynamic theory for active chiral hexatics which do not spontaneously rotate. We consider an overdamped dynamics (i.e., consider a high friction limit) and take  $f(\rho) = \rho \ln \rho$ , which implies  $\rho \nabla(\delta F/\delta \rho) = \nabla \rho$ . In detail, the linearised constitutive equation for the velocity field is

$$\begin{pmatrix} \Gamma & \Gamma_c \\ -\Gamma_c & \Gamma \end{pmatrix} \begin{pmatrix} v_x \\ v_y \end{pmatrix} = -\gamma_c K \nabla^2 \begin{pmatrix} \partial_x \theta \\ \partial_y \theta \end{pmatrix} + \frac{K}{2} \nabla^2 \begin{pmatrix} \partial_y \theta \\ -\partial_x \theta \end{pmatrix} - \begin{pmatrix} \partial_x \rho \\ \partial_y \rho \end{pmatrix} + \zeta \begin{pmatrix} \partial_y \theta \\ -\partial_x \theta \end{pmatrix} + \zeta_c \begin{pmatrix} \partial_x \theta \\ \partial_y \theta \end{pmatrix} \quad (\text{I.C.1})$$

Upon eliminating the velocity field, we obtain the coupled equations for density and angle fields:

$$\partial_t \theta = -q^2 \left[ \left( \Gamma_6 K + \frac{\Gamma_c \zeta_c - \Gamma \zeta + 2\gamma_c(\Gamma \zeta_c + \zeta \Gamma_c)}{2(\Gamma^2 + \Gamma_c^2)} \right) \theta - \frac{\Gamma_c + 2\Gamma \gamma_c}{2(\Gamma^2 + \Gamma_c^2)} \rho \right] + \xi_\theta \quad (\text{I.C.2})$$

$$\partial_t \rho = -q^2 \rho_0 \left[ -\frac{\Gamma \zeta_c + \zeta \Gamma_c}{\Gamma^2 + \Gamma_c^2} \theta + \frac{\Gamma}{\Gamma^2 + \Gamma_c^2} \rho \right] + \xi_\rho \quad (\text{I.C.3})$$

where  $\xi_\rho$  is a conserving spatiotemporally white noise whose strength  $\Delta_\rho$  is related to  $\Delta_v$  as

$$\Delta_\rho = \frac{q^2 \Delta_v}{\Gamma^2 + \Gamma_c^2} \quad (\text{I.C.4})$$

Note that in an achiral but active system, the  $\theta$  and  $\rho$  equations would have been decoupled at this order in wavevectors since the angle field can only enter the density equation through  $\nabla \cdot \mathbf{v}$  implying that the achiral active force (to which the velocity is proportional to in the overdamped limit)  $\hat{z} \times \nabla \theta$ , which is solenoidal, could only lead to a divergence-free current which would not affect the density fluctuations and the force due density fluctuations  $\propto \nabla \rho$ , being irrotational could not affect the angular fluctuations which in achiral systems could only depend on the vorticity. However, the presence of *chiral active* couplings has profound implications for the density fluctuations. These couplings yield a mass density current  $\propto \nabla \theta$  which in the steady-state must be balanced by diffusive current  $\propto \nabla \rho$  [1]. Thus, just as in active nematics, density fluctuations in chiral active hexatics must be as large as orientational fluctuations. However, orientational fluctuations are Goldstone modes of broken rotational symmetry and their static-structure factor at small wavevectors must therefore diverge as  $1/q^2$  [10]. This implies that the static structure factor of density fluctuations must also diverge at wavevectors as  $1/q^2$  in contrast to all equilibrium systems not at a critical point and achiral active hexatic systems in which the static structure factor of density fluctuations go to a constant value in the small wavevector limit. More quantitatively, the diffusive eigenfrequencies for the coupled density angle fluctuations are

$$\omega_\pm = -\frac{iq^2}{2} \left[ K\Gamma_6 + \frac{\Gamma_c \zeta_c - \Gamma \zeta + 2\gamma_c(\Gamma \zeta_c + \zeta \Gamma_c) + 2\Gamma \rho_0}{2(\Gamma^2 + \Gamma_c^2)} \pm \sqrt{\left( K\Gamma_6 + \frac{\Gamma_c \zeta_c - \Gamma \zeta + 2\gamma_c(\Gamma \zeta_c + \zeta \Gamma_c) + 2\Gamma \rho_0}{2(\Gamma^2 + \Gamma_c^2)} \right)^2 - 2 \frac{(2K\Gamma\Gamma_6 - \zeta)\rho_0}{\Gamma^2 + \Gamma_c^2}} \right] \quad (\text{I.C.5})$$

This implies that the dynamic structure factor of density fluctuations, which we can calculate by adding a conserving noise of strength  $\Delta_\rho$  to the density equation and a non-conserving noise of strength  $\Delta_\theta$  to the angular equation, is

$$\lim_{q \rightarrow 0} \langle |\rho_{q,\omega}|^2 \rangle = \frac{q^4 (\Gamma_c \zeta + \zeta_c \Gamma)^2 \rho_0^2 \Delta_\theta}{(\Gamma^2 + \Gamma_c^2)^2 |\omega - \omega_+|^2 |\omega - \omega_-|^2}. \quad (\text{I.C.6})$$

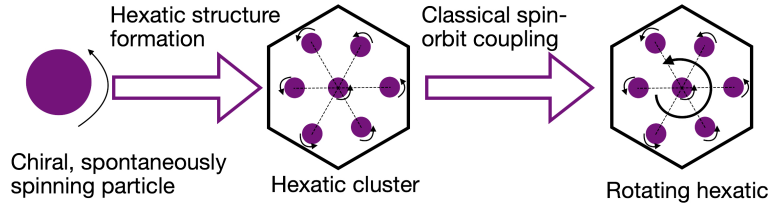

FIG. 1: Individual chiral particles rotate and when they couple to form a hexatic cluster, the cluster as a whole can rotate due to classical spin-orbit interaction.

This implies that the static structure factor

$$\langle \rho_q(t) \rho_{-q}(t) \rangle = \int_{-\infty}^{\infty} \frac{d\omega}{2\pi} \langle |\rho_{q,\omega}|^2 \rangle \propto \frac{1}{q^2} \quad (\text{I.C.7})$$

Since the static structure factor scales as  $1/q^2$  and since  $\lim_{q \rightarrow 0} \langle |\rho_q(t)|^2 \rangle \rightarrow (\delta N)^2/N$ , where  $\delta N$  is fluctuation in the number of particles in a region containing  $N$  particles on average, this implies that R.M.S. number fluctuations  $\sqrt{(\delta N)^2}$  scale as  $N$  and not as  $\sqrt{N}$  as it would in all equilibrium systems not at a critical point. Furthermore, unlike in active nematics, where the coefficient of the *anisotropic* active density current itself has to vanish at large scales in the quasi-long-range ordered (QLRO) nematic phase in two dimensions [9, 11], here the coefficient of active density current have the same symmetry as the helicity modulus in superfluids and would not vanish at large scales as long as a QLRO hexatic state existed. However, as discussed in the main text, the hexatic is itself destroyed due to nonlinearities at large scales and beyond that scale, the number fluctuations also crossover to display the usual scaling  $\sqrt{(\delta N)^2} \sim \sqrt{N}$ . Further, (I.C.2) and (I.C.3) correspond to models of particles sliding on randomly fluctuating surfaces [12], where a particle current proportional to the gradient of the height of the surface drives clustering even in the absence of attractive interactions, with  $\theta$  playing the role of the height field. It was shown in [12] that this leads to an unusual fluctuation-dominated phase ordering. Such a phase separated state may be realised here as well in the *orientationally ordered* phase with the system perpetually transitioning among many configurations with a finite number of macroscopic clusters instead of forming a single macroscopic high density cluster. However, this is not likely to lead to a macroscopic fluctuation-dominated phase-ordered state in the limit of infinite system sizes since as, discussed in the main text, the hexatic state itself is destroyed due to nonlinearities. A fluctuation-dominated phase ordered state is not possible in an infinite system even in an achiral nematic, but for a different reason – there, the active current is not a pure gradient and due to the nematic only having quasi-long-range order, the coefficient of this active current vanishes at large scale.

#### D. Linear theory of chiral active hexatic: Density-dependent rotation rate

In the last section we discussed active hexatics which do not spontaneously rotate. However, any orientational symmetry broken chiral nonequilibrium system may also spontaneously rotate. Indeed, such rotation for uniaxially ordered chiral systems have been predicted [7] and observed experimentally [8]. In such systems it was shown that active rotation has important effects on the stability of, and the fluctuations in, the ordered phase. We now consider the effect of such chiral rotation on the hexatic phase and discuss the possibility of a novel orientation-density wave.

To consider the effect of spontaneous rotation on the hexatic phase, we augment (I.A.2) with the spontaneous rotation rate  $\Omega$ . Note that this means a *local* rotation of the angle field not a global rotation of the systems as whole, i.e., individual hexatic clusters spontaneously rotate about their own centres of symmetry without any motion of the centres-of-symmetry. This can arise in multiple ways. If we consider six-fold symmetric elementary units, these units can spontaneously rotate if they are chiral. Even when the elementary units are isotropic and chiral, a six-fold symmetric structure composed of them can rotate as a whole due to classical spin-orbit coupling [15, 16]. We present a schematic of this in Fig. 1. Further, chiral structures with hexagonal symmetry, which spontaneously rotate, can also be self-assembled [16]. In addition to the rotation of the hexatic clusters about their individual centres-of-symmetry, spin-orbit coupling may also induce a global revolution of the hexatic clusters about their common centre-of mass. This would lead to a constant *vorticity*  $\nabla \times \mathbf{v}$  – corresponding to a rigid rotation of the coordinate frame. This would be an *additional* source of the change of the angle field which we do not consider here, but which can simply be taken into account by moving to the co-rotating frame. Note that such in-situ rotation of the hexatic clusters are not necessarily suppressed by steric interactions since active systems can orientationally order at lower densities than their passive counterparts [17]. A purely constant  $\Omega$  does not change the behaviour of the fluctuations discussed in the last

section (since the equations of motion have an extra symmetry under independent rotations of space and structure; this symmetry would be broken if we expanded the equations of motion to fifth order in gradients), unlike in active nematics [7]. Concretely, we can transform to a frame rotating with the hexatic phase and define the deviation from this as  $\delta\theta = \theta - \Omega t$ . The coupled equations for  $\delta\theta$  and  $\rho$  are exactly the same as (I.C.2) and (I.C.3) (this would not be case if we had expanded the equations of motion up to fifth order in gradients) and therefore, a hexatic rotating at a constant angular speed also displays giant number fluctuations. However, the rotation rate of the hexatic need not be constant. In particular, it can depend on the local density. For instance, the rotation rate may be smaller in denser regions and larger in less dense regions. In this case,  $\Omega(\rho)$  can be expanded as

$$\Omega(\rho) = \Omega(\rho)|_{\rho=\rho_0} + \frac{\partial\Omega}{\partial\rho}\bigg|_{\rho=\rho_0} \delta\rho = \Omega_0 + \Omega_1\delta\rho. \quad (\text{I.D.1})$$

Defining  $\delta\theta = \theta - \Omega_0 t$ , we therefore find that  $\partial_t\delta\theta \sim \Omega_1\delta\rho$  and  $\partial_t\rho \sim q^2\rho_0(\Gamma\zeta_c + \zeta\Gamma_c/\Gamma^2 + \Gamma_c^2)\theta$ . This implies a *linear* dispersion  $\omega = \pm cq$  where

$$c = \sqrt{-\frac{\rho_0\Omega_1(\Gamma_c\zeta + \Gamma\zeta_c)}{\Gamma^2 + \Gamma_c^2}}. \quad (\text{I.D.2})$$

When  $\Omega_1(\zeta_c\Gamma + \Gamma_c\zeta) < 0$ , i.e. either when the rotation rate slows down with increasing density and a gradient of the angle field leads to a mass current in the direction of the gradient or when the rotation rate increases with density and an angular gradient leads to a mass current in the opposite direction, this leads to a propagating density-bond-angle wave with a linear dispersion. Such linear waves, reminiscent of sound modes, in overdamped active systems are unusual. They exist in polar active systems since there polarisation also plays the role of a velocity and due to the broken rotational symmetry, mimic sound waves in underdamped fluids. Here, however, their origin is completely distinct. They arise due to the coupling of a chiral active mass current and a density-dependent rotation rate and therefore has no achiral analogue. Eq. (I.D.2) further implies that when  $\Omega_1(\zeta_c\Gamma + \Gamma_c\zeta) > 0$ , the homogeneous hexatic phase is unstable with a growth rate of fluctuations  $\propto q$ . To understand this instability, let us consider the case in which  $\Omega_1$  and  $(\zeta_c\Gamma + \Gamma_c\zeta)$  are both positive. In this case, an angular gradient leads to a mass current in the direction of the gradient leading to an increase in density. This higher density leads to a local increase of the rotation rate reinforcing the angular gradient and leading to an instability of the homogeneous hexatic state.

We now calculate the mode structure of a rotating hexatic up to  $\mathcal{O}(q^2)$  and use this to demonstrate that when the rotating hexatic is stable, it has *normal* number fluctuations as opposed to non-rotating chiral hexatics which we showed in the last section has *giant* number fluctuations.. Augmenting (I.C.2) with the term  $\Omega_1\delta\rho$  and changing the angular variable to  $\delta\theta$  instead of  $\theta$ , we obtain

$$\omega_{\pm} = \pm \sqrt{-\frac{\rho_0\Omega_1(\Gamma_c\zeta + \Gamma\zeta_c)}{\Gamma^2 + \Gamma_c^2}q} - i\frac{q^2}{2} \left[ K\Gamma_6 + \frac{\Gamma_c\zeta_c - \Gamma\zeta + 2\gamma_c(\Gamma\zeta_c + \zeta\Gamma_c) + 2\Gamma\rho_0}{2(\Gamma^2 + \Gamma_c^2)} \right] \quad (\text{I.D.3})$$

Using these, we calculate the static structure factor of density fluctuations, as in the last section, when  $\Omega_1$  and  $(\Gamma_c\zeta + \Gamma\zeta_c)$  have opposite signs:

$$\lim_{q \rightarrow 0} \langle |\delta\rho|^2 \rangle = \frac{2\Delta_{\theta}\rho_0|\Gamma_c\zeta + \Gamma\zeta_c|}{|\Omega_1|[2K\Gamma_6(\Gamma^2 + \Gamma_c^2) + \Gamma_c\zeta_c - \Gamma\zeta + 2\gamma_c(\Gamma\zeta_c + \zeta\Gamma_c) + 2\Gamma\rho_0]}. \quad (\text{I.D.4})$$

This static structure factor is independent of  $q$  at small wavevectors and therefore, does not diverge at large scales. This implies that the R.M.S. number fluctuations  $\sqrt{(\delta N)^2}$  in a region containing on average  $N$  particles scale as  $\sqrt{N}$  as in passive systems. Thus, the wave-like dispersion of coupled angular and density fluctuations suppresses the density fluctuations. Note that this mechanism of suppression of giant number fluctuations is distinct from the suppression of GNF in [2]. There, the suppression of giant number fluctuations was the result of the suppression of *angular* fluctuations in rotating phases. In contrast, here the angular fluctuations remain large (diverging as  $1/q^2$  at small  $q$ ) but the coupling of the angular fluctuations to the density via the  $\Omega_1$  term leads to the suppression of density fluctuations.

When  $\Omega_1$  and  $(\Gamma_c\zeta + \Gamma\zeta_c)$  have the same sign on the other hand, the homogenous hexatic state is unstable as discussed earlier. In this case we expect an inhomogeneous state with the characteristic lengthscale

$$L_c = \left[ \frac{K\Gamma_6\sqrt{(\Gamma^2 + \Gamma_c^2)}}{2\sqrt{\rho_0\Omega_1(\Gamma_c\zeta + \Gamma\zeta_c)}} + \frac{\Gamma_c\zeta_c - \Gamma\zeta + 2\gamma_c(\Gamma\zeta_c + \zeta\Gamma_c) + 2\Gamma\rho_0}{4\sqrt{(\Gamma^2 + \Gamma_c^2)}\sqrt{\rho_0\Omega_1(\Gamma_c\zeta + \Gamma\zeta_c)}} \right] \quad (\text{I.D.5})$$

assuming that the coefficient of the  $\mathcal{O}(q^2)$  term in (I.D.3) is stabilising.



### E. Fluctuations of a hexatic suspended in a momentum-conserved incompressible fluid

We now consider a hexatic phase formed by active particles suspended in a momentum-conserved incompressible fluid. The density of active particles is denoted by  $\rho$  as earlier, while the joint density of the particles and the fluid is controlled by the incompressibility constraint  $\nabla \cdot \mathbf{v} = 0$  where  $\mathbf{v}$  is now the centre-of-mass velocity field of the particles and the fluid. The equation of motion for the bond angle field for a non-rotating hexatic is

$$\partial_t \theta = \frac{1}{2} \epsilon_{ij} \partial_i v_j + \Gamma_6 K \nabla^2 \theta \quad (\text{I.E.1})$$

which differs from (I.A.2) only through the absence of the term proportional to  $\nabla \cdot \mathbf{v}$  which vanishes due to incompressibility. The Stokes equation in this case is

$$\eta \nabla^2 \mathbf{v} = \nabla \Pi + \frac{K}{2} (\hat{z} \times \nabla) \nabla^2 \theta, \quad (\text{I.E.2})$$

where  $\Pi$  is the pressure that enforces the incompressibility constraint. Note that there is no active force in this equation – the forces  $\propto \zeta$  nor  $\propto \zeta_c$  are not allowed in momentum-conserved, incompressible fluids. Since the momentum equation for active hexatic suspensions in a momentum-conserved, incompressible fluid does not contain any active force, there is no analogue of generic instability of uniaxial suspensions for hexatic systems and the angular dynamics reduces to

$$\partial_t \theta = K \left( \Gamma_6 + \frac{1}{4\eta} \right) \nabla^2 \theta. \quad (\text{I.E.3})$$

which implies that the angular dynamics is purely passive. The equation for the *concentration* of the active units however contains a chiral active current  $\propto \nabla \theta$ :

$$\partial_t \rho = \zeta_\rho \nabla^2 \theta + D_\rho \nabla^2 \rho \quad (\text{I.E.4})$$

where  $\zeta_\rho$  is the phenomenological coefficient for the active current and  $D_\rho$  is a diffusion constant. The driving of the density due to the active current leads to giant number fluctuations of density in this case as well, with the static structure factor  $\lim_{q \rightarrow 0} \langle |\delta \rho|^2 \rangle \propto 1/q^2$ . To the best of our knowledge, active chiral hexatics constitute the only example of an active suspension in a momentum-conserved, incompressible fluid that displays giant number fluctuations.

Considering a rotating chiral hexatic, with a density-dependent angular speed  $\Omega = \Omega_0 + \Omega_1 \delta \rho$ , we obtain either a wave with a linear dispersion and speed  $\sqrt{\zeta_\rho \Omega_1}$  or an instability that grows linearly with the wavevector just as in Sec. IB, and a consequent suppression of giant number fluctuations in the stable ordered phase. This concludes our discussion of the linear theory of the ordered chiral hexatic.

### F. Dynamics of a single disclination in the hexatic phase

In this section we present the detailed calculation of the dynamics of a single disclination in active chiral hexatics. The full order parameter of the hexatic is

$$\Psi = \psi e^{i6\theta} \quad (\text{I.F.1})$$

whose dynamics that reduces to (I.A.2) when  $\psi = 1$  is (see [32])

$$\partial_t \Psi + \mathbf{v} \cdot \nabla \Psi = \frac{i}{2} \Psi \epsilon_{ij} \partial_i v_j + \Gamma_6 K \left[ \nabla^2 \Psi + \frac{1}{\zeta^2} \Psi (1 - |\Psi|^2) \right] \quad (\text{I.F.2})$$

The zero activity solution of a  $+1/6$  disclination is

$$\Psi_0 = \psi_0 e^{i\phi}; \quad \nabla^2 \Psi_0 = 0; \quad \mathbf{v}_0 = 0 \quad (\text{I.F.3})$$

where  $\phi$  is the azimuthal angle. We now calculate the perturbation to this solution due to small activity. We take all active coefficients  $\Gamma_c$ ,  $\zeta$  and  $\zeta_c$  to be  $\mathcal{O}(\Delta\mu)$  and define  $\Psi = \Psi_0 + \Delta\mu \Psi_1$ ,  $\mathbf{v} = \mathbf{v}_0 + \Delta\mu \mathbf{v}_1$ . Assuming a quasi-static dynamics for the disclination we can write

$$(\mathbf{v}_1 - \mathbf{v}_d) \cdot \nabla \Psi_0 + \omega_d \mathbf{r} \times \nabla \Psi_0 - \frac{i}{2} \epsilon : (\nabla \mathbf{v}_1) \Psi_0 = \mathcal{I} = [\nabla^2 \Psi_1 + \{\Psi_1 (1 - 2|\Psi_0|^2) - \Psi_0^2 \Psi_1^*\}] \quad (\text{I.F.4})$$

in the co-moving and co-rotating frame of the defect, where  $\mathbf{v}_d$  and  $\omega_d$  are the defect translational and angular speed and we have rescaled space by  $\varsigma$  and time by  $\varsigma^2/K\Gamma_6$ . The operator operating on  $\Psi_1$  has three zero eigenvalues [29, 31], as usual in all such problems, two corresponding to translations  $\Phi = \nabla\Psi_0$  and one corresponding to rotation  $\Phi = i\Psi_0$  (corresponding to rotation and translation invariance of the problem). Therefore, we have the usual solvability condition

$$\text{Re} \left[ \int_{\Xi} d^2r \mathcal{I} \Phi^* \right] = \text{Re} \left[ \oint_{\partial\Xi} \Phi^* \partial_{\perp} \Psi_1 - \Psi_1 \partial_{\perp} \Phi^* \right] \quad (\text{I.F.5})$$

where  $\Xi$  is a region of space and  $\partial_{\perp}$  is the normal derivative to its boundary  $\partial\Xi$ . Note that the only point of difference between this model and standard hexatics arises from the active force which we take to only depend on  $\theta$  (one could easily take it to depend on the whole order parameter  $\Psi$ , as is done in nematic liquid crystal, [29, 31], but that wouldn't change the qualitative results). For a positive disclination,

$$\nabla\Psi_0 = e^{i\phi} \left[ \partial_r \psi \begin{pmatrix} \cos \phi \\ \sin \phi \end{pmatrix} + \frac{i\psi}{r} \begin{pmatrix} \sin \phi \\ -\cos \phi \end{pmatrix} \right]. \quad (\text{I.F.6})$$

The active velocity for a positive disclination is

$$\mathbf{v} = \frac{\psi_0}{r\Gamma} [(\zeta \cos \phi - \zeta_c \sin \phi) \hat{x} + (\zeta_c \cos \phi + \zeta \sin \phi) \hat{y}] \quad (\text{I.F.7})$$

where we have explicitly shown the dependence on  $\psi_0$ , which vanishes as  $r$  as  $r \rightarrow 0$  and goes to 1 as  $r \rightarrow \infty$ . Note that  $\epsilon : (\nabla\mathbf{v}_1)$  is identically 0. Note that  $\Gamma_c$  does not appear in this expression which is at  $\mathcal{O}(\Delta\mu)$ . We see by projecting on to the translational part (i.e., multiplying  $\mathcal{I}$  by  $(\nabla\Psi_0)^*$  and integrating) that all integrals containing the flow vanish. This implies that the disclination is not self-advected and only moves due to the gradients of  $\theta$  created by other disclinations (or a smooth variation of  $\theta$ ) just as in equilibrium systems. This is expected since there is no vectorial symmetry breaking in a hexatic defect. Therefore, the translational dynamics of disclinations in a chiral hexatic is not distinct from a passive system. However,

$$\text{Re} \left[ \int d^2r \mathbf{v}_1 \cdot \nabla\Psi_0 (i\Psi_0)^* \right] = \text{Re} \left[ \int d^2r \mathbf{v}_1 \cdot \nabla\Psi_0 (-ie^{-i\phi}) \right] \neq 0 = - \int dr \frac{\psi^2}{r^2} \frac{2\pi\zeta_c}{\Gamma} \quad (\text{I.F.8})$$

Since

$$\text{Re} \left[ \int d^2r \omega_d \mathbf{r} \times \nabla\Psi_0 (-ie^{-i\phi}) \right] = -\omega_d \int dr \psi^2 2\pi, \quad (\text{I.F.9})$$

this implies that though the disclination does not move spontaneously, it rotates spontaneously with

$$\omega_d = -\frac{\zeta_c}{\gamma_r} \quad (\text{I.F.10})$$

where  $\gamma_r$  is the rotational mobility. The orientation field around a disclination lacks circular symmetry and therefore, this is non-trivial effect. Note that  $\zeta_c$  would not have affected the dynamics in an incompressible system since it yields a force  $\propto \nabla\theta$ . This implies that this rotation of disclination is suppressed in incompressible fluids. Though we have only displayed the calculation for a positive 1/6 disclination, a negative 1/6 disclination rotates with the same speed but in the opposite direction i.e., with  $\omega_d = \zeta_c/\gamma_r$ . This rotation of the pattern around the defect core does not affect the centre-of-mass motion of the disclinations.

We now present a heuristic discussion of the (lack of) self-propulsion of defects in a chiral hexatic. We will use the notation introduced in Sec. IB for this. It is known (and intuitively clear) that for a defect to self-propel, it must create a force density distribution which has an angular structure of a monopole i.e., its angular average should not vanish. We write the active force  $\mathbf{f} = f_x \hat{x} + f_y \hat{y}$  as a complex number  $f = f_x + if_y$ . The two active forces in the hexatic then can be written as  $-(\zeta/6)\Psi^* \nabla\Psi$  and  $-i(\zeta_c/6)\Psi^* \nabla\Psi$  where  $\nabla = \partial_x + i\partial_y$  and  $\nabla^* = \partial_x - i\partial_y$ . We now insert the solution of a +1/6 defect  $\theta = \phi/6$ , where  $\phi$  is the azimuthal angle. Then,

$$\Psi^* \nabla\Psi = \frac{e^{i\phi}}{r} \quad (\text{I.F.11})$$

where  $r$  is the radial coordinate in polar coordinates  $r = \sqrt{x^2 + y^2}$  and  $\phi = \tan^{-1}(y/x)$ . The chiral far-field active force due a +1/6 defect at the origin is  $i\Psi^* \nabla\Psi = ie^{i\phi}/r$ . Similarly, a -1/6 defect simply leads to the active achiral and

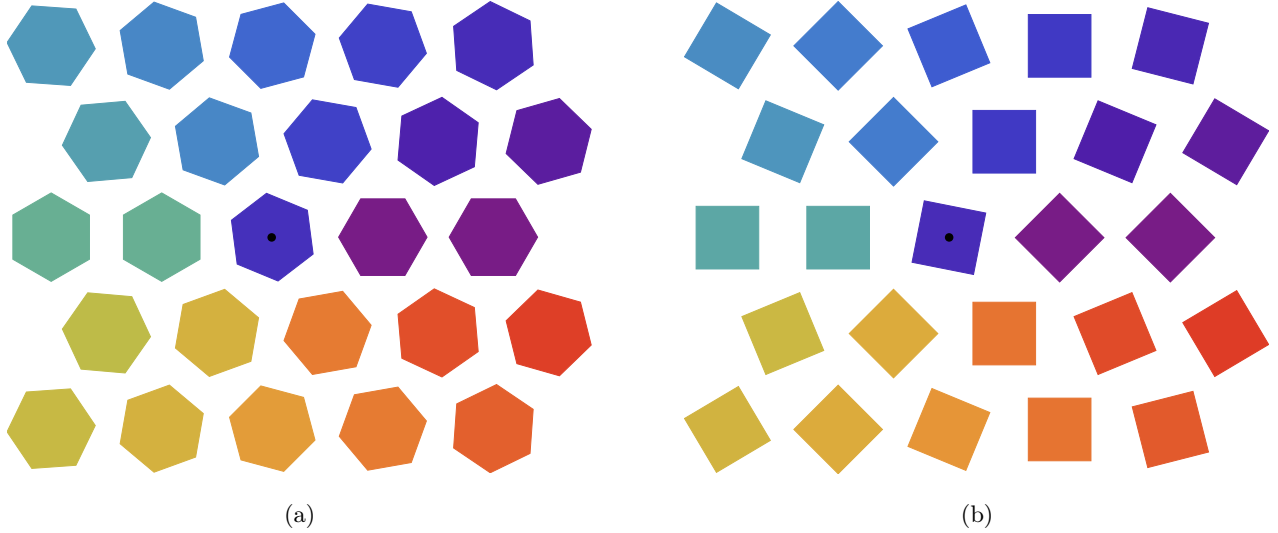

FIG. 2: (a)  $+5/6$  hexatic defect and (b)  $+3/4$  tetratic defect. The colour-map corresponds to the local angle field and is intended to guide the eye. Both of these defects have polar structures and would self-propel. However, they are likely to break up into  $5 +1/6$  defects and  $3 +1/4$  defects respectively.

chiral far-field forces  $\Psi^* \nabla \Psi = -e^{i\phi}/r$  and  $i\Psi^* \nabla \Psi = -ie^{i\phi}/r$  respectively (note that this is the far-field force density; there is no divergence of the force as  $r \rightarrow 0$  since at the origin,  $\psi_0 \rightarrow 0$  i.e., the order parameter *magnitude* vanishes at the core of the defect). It is therefore clear that neither of the active forces retained in our work can lead to self-propulsion of defects (since the angular averages of the force density for both  $\pm 1/6$  defects are 0). However, as pointed out earlier, these force densities are present in active chiral nematics as well. Even in that case, where it is known that a  $+1/2$  defect self-propels, these active terms lead to force densities whose angular average is 0. Defining a  $+1/2$  defect as  $\theta = \phi/2$  with the nematic order parameter as  $\Psi_2 = \psi e^{i2\theta}$ ,  $\Psi_2^* \nabla \Psi_2 = e^{i\phi}/r$  and  $i\Psi_2^* \nabla \Psi_2 = ie^{i\phi}/r$ . Similarly, for  $-1/2$  defect,  $\theta = -\phi/2$ ,  $\Psi_2^* \nabla \Psi_2 = -e^{i\phi}/r$  and  $i\Psi_2^* \nabla \Psi_2 = -ie^{i\phi}/r$ . This is related to the fact that these forces preserve a symmetry under independent rotations of space and spin. Instead, self-propulsion of nematic  $+1/2$  defects is due to active forces that explicitly break this symmetry:  $\nabla^* \Psi_2$  (achiral) and  $i\nabla^* \Psi_2$  (chiral). For a  $+1/2$  defect, i.e.,  $\theta = \phi/2$ ,  $\nabla^* \Psi_2 = 1/r$  and  $i\nabla^* \Psi_2 = i/r$  neither of which vanishes upon an angular integration. In contrast,  $-1/2$  defects, which have a triaxial symmetry, lead to force densities  $\nabla^* \Psi_2 = -e^{-2i\phi}/r$  and  $i\nabla^* \Psi_2 = -ie^{-2i\phi}/r$  and do not lead to any self-propulsion. One may then expect that considering terms that break the symmetry under independent space-spin rotation to one under only under joint rotations of space and spin in a chiral hexatic would lead to self-propulsion of hexatic defects as well. Such terms appear at fifth order in gradients in the hexatic (unlike the first order in gradients as in a nematic) but if they did lead to self-propulsion of defects they ought to be considered. However, even the fifth order in gradients active forces that break the independent space-spin rotation symmetry in active chiral hexatics  $\nabla^* \nabla^* \nabla^* \nabla^* \nabla^* \Psi$  (achiral) and  $i\nabla^* \nabla^* \nabla^* \nabla^* \nabla^* \Psi$  (chiral) do not lead to self-propulsion of  $+1/6$  and  $-1/6$  defects in a chiral hexatic. For a  $+1/6$  defect,  $\nabla^* \nabla^* \nabla^* \nabla^* \nabla^* \Psi \propto -e^{-4i\phi}/r^5$  and  $i\nabla^* \nabla^* \nabla^* \nabla^* \nabla^* \Psi \propto -ie^{-4i\phi}/r^5$  while for a  $-1/6$  defect  $\nabla^* \nabla^* \nabla^* \nabla^* \nabla^* \Psi \propto e^{-6i\phi}/r^5$  and  $i\nabla^* \nabla^* \nabla^* \nabla^* \nabla^* \Psi \propto ie^{-6i\phi}/r^5$ . The angular average of these vanish and therefore they do not lead to self-propulsion. This is expected based on far-field angle fields of the  $\pm 1/6$  defects: a  $+1/6$  defect has a pentagonal symmetry and a  $-1/6$  defect has a heptagonal symmetry as shown in the main text. There is a hexatic defect with charge  $+5/6$  (see Fig. 4) that self-propels with  $\nabla^* \nabla^* \nabla^* \nabla^* \nabla^* \Psi \propto -1/r^5$  and  $i\nabla^* \nabla^* \nabla^* \nabla^* \nabla^* \Psi \propto -i/r^5$ . However, a  $+5/6$  defect is likely to break into  $5 +1/6$  defects and therefore, we do not consider its dynamics. Similar analysis can be performed for active chiral triatic and tetratic defects. To summarise this section, the most abundant defects in hexatics  $\pm 1/6$  do not self-propel due to activity but do spontaneously rotate due to a combination of activity and chirality.

### G. Structure of a single defect

In the last section we demonstrated that a defect in a chiral hexatic spontaneously rotates. However, that calculation was performed within a perturbative treatment which implicitly assumed an equilibrium-like angle field due to a defect. In this section, we go beyond this and, within a treatment in which the velocity field is eliminated in favour of the

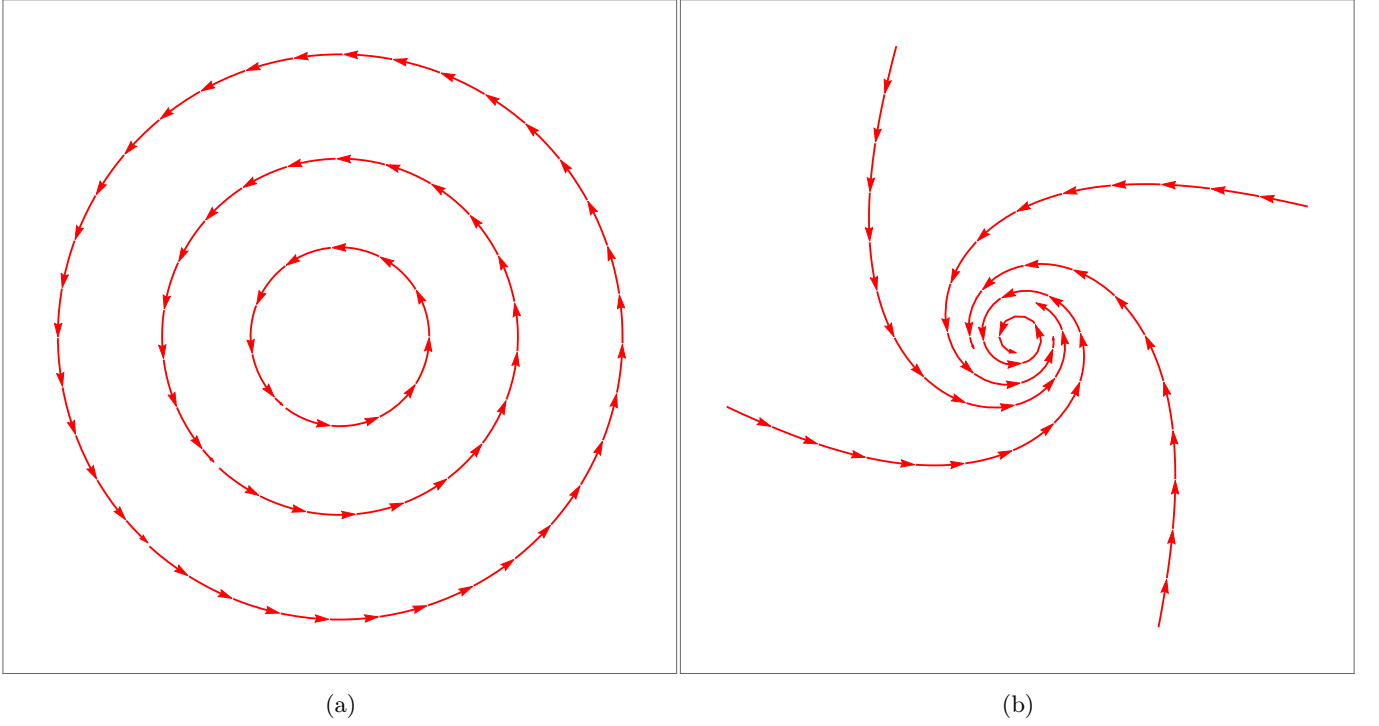

FIG. 3: (a)  $\nabla\theta$  for a  $+1/6$  defect in a passive hexatic (i.e. when  $\lambda = 0$ ). (b)  $\nabla\theta$  for a  $+1/6$  defect in a *chiral* hexatic. The vortex-like configuration of  $\nabla\theta$  due to a defect in an achiral hexatic is modified to spiral in a chiral hexatic.

This spiral structure is itself chiral and rotates at a constant rate even when the background does not rotate spontaneously.

angle field, we find the structure of the angle field due to a defect. We start with the equation for the angle field

$$\partial_t \theta = \frac{\lambda}{2} (\nabla\theta)^2 + \bar{K} \nabla^2 \theta - \omega_0 \quad (\text{I.G.1})$$

where we retain an explicit rotation rate  $\omega_0$ . This doesn't imply that this calculation *only* applies to a spontaneously rotating hexatic state, however. As discussed above, a defect in a chiral hexatic, i.e., a defect solution of this equation, spontaneously rotates even if the defect-free hexatic angle-field doesn't, and  $\omega_0$  is this rotation rate. Our calculation will explicitly demonstrate that there is no static defect solution i.e. defect solutions require  $\Omega \neq 0$ , which is consistent with the calculation in the last section.

We take a vortex solution at the origin for a  $+1/6$  defect (the calculation for  $-1/6$  defect is obvious), in the polar coordinate, as

$$\theta(r, \phi) = \frac{\phi}{6} + R(r) \quad (\text{I.G.2})$$

which leads to an equation for  $R$

$$\left( R'' + \frac{R'}{r} \right) + \tilde{\lambda} \left( \frac{1}{36r^2} + R'^2 \right) - \frac{\omega_0}{\bar{K}} = 0 \quad (\text{I.G.3})$$

where  $\tilde{\lambda} = \lambda/2\bar{K}$  and the prime denotes differentiation with respect to  $r$ . Using the Cole-Hopf transformation  $f = e^{\tilde{\lambda}R}$ , with  $f > 0$ , this equation can be linearised

$$f'' + \frac{f'}{r} + \frac{\tilde{\lambda}^2 f}{36r^2} - \frac{\tilde{\lambda} \omega_0 f}{\bar{K}} = 0. \quad (\text{I.G.4})$$

Now, if we take  $\omega_0 = 0$ , i.e., assume that the defect is not rotating, we do find a solution

$$f = C_1 \cos \left[ \frac{\tilde{\lambda}}{6} \ln \left( \frac{r}{\varsigma} \right) \right] + C_2 \sin \left[ \frac{\tilde{\lambda}}{6} \ln \left( \frac{r}{\varsigma} \right) \right] \quad (\text{I.G.5})$$

where  $C_1$ ,  $C_2$  and  $\varsigma$  are constants. This would seem to suggest that a non-rotating defect solution is possible in a chiral hexatic. However, as pointed out in [35], this oscillatory function does not yield a real value for  $R = \ln f/\tilde{\lambda}$  for all  $r > 0$  and therefore, cannot describe a physical defect solution. Therefore, only solutions with  $\omega_0 \neq 0$  are allowed. These solutions are in terms of the modified Bessel functions. We expect the solution to be bounded as  $r \rightarrow \infty$  and the solution that compatible with this is in terms of the Bessel function of the *second* kind  $K_{i\tilde{\lambda}/6} \left( r\sqrt{\tilde{\lambda}\omega_0/\bar{K}} \right)$ . This

behaves as  $f(r) \sim e^{-r\sqrt{\tilde{\lambda}\omega_0/\bar{K}}}/\sqrt{r}$  beyond a maximum at  $r = r_0 = \sqrt{\bar{K}}e^{(-\pi/2\tilde{\lambda})}/\sqrt{\tilde{\lambda}\omega_0}$  while at shorter scales the function becomes oscillatory. However, short-scale structure of a defect cannot be obtained using only the equation for the angle-field – the amplitude equation, as in the last section, has to be retained for the core structure of the defect. The scale  $r_0$ , which is the core-radius of the defect, however can be inverted to obtain an estimate for  $\omega_0$  – which is the steady rotation rate of the defect. The solution of  $\theta$  for large  $r$  can also be obtained from  $f$  by inverting the Cole-Hopf transformation

$$\theta(r, \phi) = -\sqrt{\frac{\omega_0}{\tilde{\lambda}\bar{K}}}r - \frac{1}{2\tilde{\lambda}} \ln \left( \frac{2r}{\pi} \sqrt{\frac{\tilde{\lambda}\omega_0}{\bar{K}}} \right) + \frac{\phi}{6} + \mathcal{O}\left(\frac{1}{r}\right). \quad (\text{I.G.6})$$

This implies that the angle field has a spiral structure. This implies that the far-field structure of the angle-field of a defect is fundamentally modified due to chirality and activity, which leads to both non-zero  $\tilde{\lambda}$  and non-zero  $\omega_0$ , and now depends explicitly on  $r$ . This is in contrast to the assumption in the last section where the only spatial dependence was within the defect-core, but for large  $r$ , the angle field was only  $\theta(r, \phi) = \phi/6$ .

## H. Defect interactions

In this section, we will consider the dynamics of a defect in the presence of other defects. We will focus primarily on the two-defect interaction. As pointed out in the main text, defects unbind in the hexatic phase at arbitrarily low noise. We will establish this now directly by calculating the interaction between defects and also demonstrate that this interaction is *non-mutual*. Note that non-mutual interaction between defects is not a speciality of chiral active hexatics but a feature of all active ordered phases including active nematics and polar systems.

The phase gradient at the site of the  $i$ -th defect due to all other defects is given by

$$\nabla\theta = -\epsilon \cdot \nabla_{\mathbf{r}_i} \sum_{j \neq i} s_j \ln \left| \frac{\mathbf{r}_i - \mathbf{r}_j}{\varsigma} \right|. \quad (\text{I.H.1})$$

This phase gradient induces a flow. The flow induced by other defects or smooth gradients is assumed not to vary over the scale of the core of the defect [29]. The velocity induced at the site of the  $i$ -th defect due to active forces generated by the presence of phase gradients due to other defects or smooth bond-angle distortions is

$$\mathbf{v}(\mathbf{r}_i) = \frac{1}{\Gamma} [\zeta\epsilon \cdot \nabla\theta|_{\mathbf{r}=\mathbf{r}_i} + \zeta_c \nabla\theta|_{\mathbf{r}=\mathbf{r}_i}]. \quad (\text{I.H.2})$$

A defect will be entrained by this flow which is generated by all other defects or smooth distortions of the angle field. In addition, the elastic interactions with other defects leads to a force on the  $i$ -th defect [25]. Including this, we obtain the Langevin equation for the position of the  $i$ -th defect:

$$\dot{\mathbf{r}}_i = \frac{1}{\Gamma} [\zeta\epsilon \cdot \nabla\theta|_{\mathbf{r}=\mathbf{r}_i} + \zeta_c \nabla\theta|_{\mathbf{r}=\mathbf{r}_i}] + 2\pi\mu s_i \bar{K}\epsilon \cdot (\nabla\theta)|_{\mathbf{r}=\mathbf{r}_i} - 2\pi\mu_c s_i \bar{K}\epsilon \cdot (\epsilon \cdot (\nabla\theta)|_{\mathbf{r}=\mathbf{r}_i}) + \chi. \quad (\text{I.H.3})$$

Here,  $s_i = \pm 1/6$  is the charge of the  $i$ -th defect,  $\mu$  is a standard mobility (which should actually depend on the speed of the defect, but which we take to be constant) and  $\chi$  is a Gaussian white noise whose strength is  $2T\mu$ . We have also included a further chiral active mobility  $\mu_c$ . This is generically allowed in this system by symmetry. Notice that the terms due to  $\mathbf{v}$  affect both  $+$  and  $-$  defects symmetrically, while the elastic force terms, as usual, depend on the sign of the defect. If we ignore the nonlinear term  $\propto \lambda$  in the equation of motion for  $\theta$ , this yields the equation of motion for the position of a  $+1/6$  disclination in the presence of a  $-1/6$  disclination as

$$\dot{\mathbf{r}}_+ = - \left[ \frac{1}{6\Gamma} (\zeta\mathbf{l} - \zeta_c\epsilon) + \frac{\pi\bar{K}}{18} (\mu\mathbf{l} - \mu_c\epsilon) \right] \cdot \nabla_{\mathbf{r}_+} \ln \left| \frac{\mathbf{r}_+ - \mathbf{r}_-}{\varsigma} \right| + \chi \quad (\text{I.H.4})$$

where  $\mathbf{r}_+$  and  $\mathbf{r}_-$  denote the positions of the  $+1/6$  and  $-1/6$  disclinations respectively. However, as argued in the main text, the theory ignoring the nonlinearity is incorrect: the nonlinear coupling modifies the interaction strength

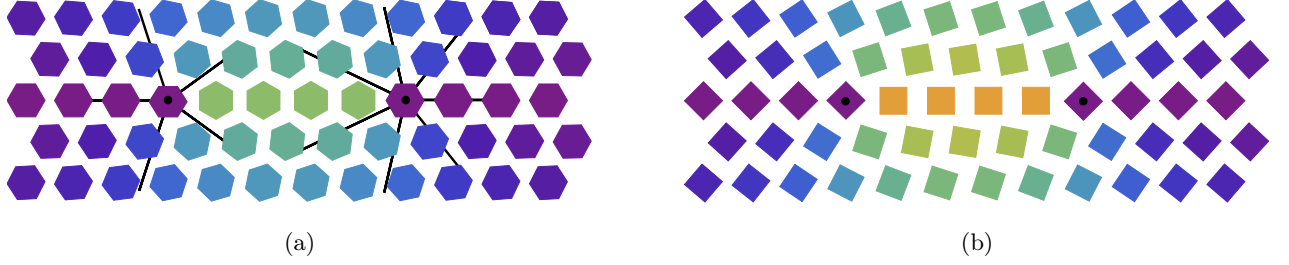

FIG. 4: (a)  $\pm 1/6$  hexatic defect pair ( $+1/6$  on the left and  $-1/6$  on the right) and (b)  $\pm 1/4$  tetratic defect pair ( $+1/4$  on the left and  $-1/4$  on the right). The colour-map corresponds to the local angle field and is intended to guide the eye. The defect positions are denoted by black dots. Both of these defect *pairs* self-propel.

between disclinations. Therefore, we now closely follow the calculation presented in [36] for defects in compact KPZ equation to calculate the correction to (I.H.4) due to  $\lambda$ . We will consider  $\lambda$ , the coefficient of  $(\nabla\theta)^2/2$  term in the equation of motion of the angle field, to be free-parameter, unlike in the main text where we obtained it from the  $\mathbf{v} \cdot \nabla\theta$  advective nonlinearity. This is justified since a nonlinearity of this form is not constrained to arise only advection. Instead, it can also arise directly in the equation of motion for  $\theta$ . The primary difference between the model considered here and in [36] arises from (I.H.3) – the terms  $\propto \mu_c, \zeta_c$  are absent in their Langevin equation for the defect position. Additionally, they did not consider the entrainment of defects due to an active flow and therefore, the term  $\propto \zeta$  was also absent in their work. Taking into account these differences, we obtain the  $\mathcal{O}(\lambda/\bar{K})$  correction to the velocity of the  $+1/6$  defect:

$$\mathbf{v}_+^{(1)} = \left[ \frac{1}{\bar{K}\Gamma} (\zeta \mathbf{I} - \zeta_c \boldsymbol{\epsilon}) + \frac{\pi}{3} (\mu \mathbf{I} - \mu_c \boldsymbol{\epsilon}) \right] \cdot \frac{\lambda}{64} \frac{\boldsymbol{\epsilon} \cdot (\mathbf{r}_+ - \mathbf{r}_-)}{|\mathbf{r}_+ - \mathbf{r}_-|^2} \left[ 2 \ln \left| \frac{\mathbf{r}_+ - \mathbf{r}_-}{\varsigma} \right| - \frac{1}{2} \right]. \quad (\text{I.H.5})$$

Note that while in [36], the first order correction only leads to motion perpendicular to  $\mathbf{r}_+ - \mathbf{r}_-$ , here, there is a component of the velocity along  $\mathbf{r}_+ - \mathbf{r}_-$  as well, stemming from the explicitly chiral terms. A heuristic explanation for this can be provided based on a single defect solution of the static compact KPZ equation. In polar coordinates, a defect solution at the origin will have  $(\nabla\theta)_\varphi \sim 1/r$ , where  $r$  is the radial coordinate and  $\varphi$  is the azimuthal coordinate. It can be shown that a  $\nabla\theta$  whose azimuthal component is  $\sim 1/r$  must have a radial component at large  $r$ ,  $(\nabla\theta)_r \sim -(\lambda/r) \ln r$ . In the achiral model considered in [36], the force is  $\propto \boldsymbol{\epsilon} \cdot \nabla\theta$  and therefore,  $(\nabla\theta)_\varphi$  leads to the usual  $1/r$  radial force due the defect, while  $(\nabla\theta)_r$  leads to a purely azimuthal force. The contribution to the radial force in their calculation appears only at second order in  $\lambda$ , which explicitly involves interactions between two defects. However, in a chiral and active system the mobility tensor is allowed to have an antisymmetric part and chiral active forces are present as well. This allows the Langevin equation for the position of the defect to have active, chiral terms  $\propto \nabla\theta$ . This leads to a contribution  $\propto \ln r/r$  in the radial direction at first order in the nonlinearity.

The second order correction to the velocity of a  $+1/6$  defect due to the presence of a  $-1/6$  defect can also be calculated following [36]:

$$\mathbf{v}_+^{(2)} = \left[ \frac{1}{\Gamma} (\zeta \mathbf{I} - \zeta_c \boldsymbol{\epsilon}) + \frac{\pi \bar{K}}{3} (\mu \mathbf{I} - \mu_c \boldsymbol{\epsilon}) \right] \cdot \frac{1}{48} \left( \frac{\lambda}{12\bar{K}} \right)^2 \frac{(\mathbf{r}_+ - \mathbf{r}_-)}{|\mathbf{r}_+ - \mathbf{r}_-|^2} \left[ 8 \ln \left| \frac{\mathbf{r}_+ - \mathbf{r}_-}{\varsigma} \right|^2 + 4 \left| \frac{\mathbf{r}_+ - \mathbf{r}_-}{\varsigma} \right| - 1 \right]. \quad (\text{I.H.6})$$

We now collect all terms that lead to attraction or repulsion between a  $\pm 1/6$  pair. The velocity of a  $+1/6$  defect in the presence of a  $-1/6$  defect along the line joining the  $\pm 1/6$  defect is

$$\begin{aligned} \dot{r}_{+-}^{\parallel} = - \left[ \left\{ \frac{\zeta}{6\Gamma} + \frac{\pi \bar{K} \mu}{18} \right\} - \left\{ \frac{\zeta_c}{\bar{K}\Gamma} + \frac{\pi \mu_c}{3} \right\} \right] \frac{\lambda}{64} \left\{ 2 \ln \left| \frac{r_{+-}}{\varsigma} \right| - \frac{1}{2} \right\} \\ - \left\{ \frac{\zeta}{\Gamma} + \frac{\pi \bar{K} \mu}{3} \right\} \frac{1}{48} \left( \frac{\lambda}{12\bar{K}} \right)^2 \left\{ 8 \ln \left| \frac{r_{+-}}{\varsigma} \right|^2 + 4 \left| \frac{r_{+-}}{\varsigma} \right| - 1 \right\} \frac{1}{r_{+-}} \end{aligned} \quad (\text{I.H.7})$$

where  $r_{+-}$  is a shorthand for  $|\mathbf{r}_+ - \mathbf{r}_-|$ ,  $\hat{\mathbf{r}}_{+-}$  is the unit-vector from  $-1/6$  defect to the  $+1/6$  defect and  $\dot{r}_{+-}^{\parallel} = \hat{\mathbf{r}}_{+-} \cdot \dot{\mathbf{r}}_+$ . The deterministic part of the equation of motion of a  $-1/6$  defect due to a  $+1/6$  defect is not simply the negative of

(I.H.7) however – the interactions between defects are not governed by a potential – but has the form

$$\begin{aligned} \dot{r}_{-}^{\parallel} = & - \left[ \left\{ \frac{\zeta}{6\Gamma} - \frac{\pi\bar{K}\mu}{18} \right\} - \left\{ \frac{\zeta_c}{\bar{K}\Gamma} - \frac{\pi\mu_c}{3} \right\} \frac{\lambda}{64} \left\{ 2\ln \left| \frac{r_{+-}}{\varsigma} \right| - \frac{1}{2} \right\} \right. \\ & \left. - \left\{ \frac{\zeta}{\Gamma} - \frac{\pi\bar{K}\mu}{3} \right\} \frac{1}{48} \left( \frac{\lambda}{12\bar{K}} \right)^2 \left\{ 8\ln \left| \frac{r_{+-}}{\varsigma} \right|^2 + 4 \left| \frac{r_{+-}}{\varsigma} \right| - 1 \right\} \right] \frac{1}{r_{+-}} \quad (\text{I.H.8}) \end{aligned}$$

where  $\dot{r}_{-}^{\parallel} = \hat{\mathbf{r}}_{+-} \cdot \dot{\mathbf{r}}_{-}$ . Notice that at the zeroth order in  $\lambda$ , a  $-1/6$  defect pulls in a  $+1/6$  defect (as well as a  $-1/6$  defect) due to the active velocity generated by the term  $\propto \zeta$  while a  $+1/6$  defect repels both  $+1/6$  and  $-1/6$  defects due to the same term. This implies that while a single  $+1/6$  or  $-1/6$  defect doesn't self-propel, a  $\pm 1/6$  defect pair acts like a pump (pulling in fluid at the minus end and pushing it out at the plus end) leading to self-propulsion. Similarly, in a tetratic, a  $\pm 1/4$  defect pairs self-propels.

The relative separation between a  $\pm 1/6$  defect pair can be calculated by subtracting (I.H.8) from (I.H.7), we can find a differential equation for the separation between a  $\pm 1/6$  pair:

$$\dot{r}_{+-} = -2 \left[ \frac{\pi\bar{K}\mu}{18} - \frac{\pi\mu_c}{3} \frac{\lambda}{64} \left\{ 2\ln \left| \frac{r_{+-}}{\varsigma} \right| - \frac{1}{2} \right\} - \frac{\pi\bar{K}\mu}{3} \frac{1}{48} \left( \frac{\lambda}{12\bar{K}} \right)^2 \left\{ 8\ln \left| \frac{r_{+-}}{\varsigma} \right|^2 + 4 \left| \frac{r_{+-}}{\varsigma} \right| - 1 \right\} \right] \frac{1}{r_{+-}} \quad (\text{I.H.9})$$

This is similar to the result obtained by [36] for the compact KPZ equation. The only difference comes from the term  $\propto \mu_c$  which was absent in [36] and yields a *first-order* in  $\lambda$  correction to the relative speed of the  $\pm 1/6$  defect pair. However, similar to that calculation, the relative speed is dominated by the term  $\propto \ln |r_{+-}|^2 / r_{+-}$ . Since this term is repulsive (for  $\bar{K} > 0$ ), this means that at large scales, a  $+1/6$  and a  $-1/6$  defect always separates, thereby destroying the ordered phase. However, this is a perturbative calculation in  $\lambda$  and higher order corrections to  $\lambda$  may dominate. If all such higher order corrections also tended to lead to unbinding of the  $\pm 1/6$  pair, then the defects would always unbind in large enough systems, destroying the ordered state. However, the strength of these corrections would not only depend on  $\bar{K}$  (which needs to be positive for the linear stability of the hexatic phase) but also on  $\mu_c$  – unlike in [36]. This makes it difficult to predict the sign of the relative velocity with distance – it could, in principle, be an oscillatory function of the the distance of separation – and therefore, difficult, without further analysis, to predict the fate of defect-unbinding transition. Furthermore, two  $+1/6$  defects and two  $-1/6$  defects have different interactions. The speed of a  $-1/6$  defect in the presence of another  $-1/6$  defect, along the line joining the two defects, is

$$\begin{aligned} \dot{r}_1^{\parallel} = & - \left[ \left\{ \frac{\zeta}{6\Gamma} - \frac{\pi\bar{K}\mu}{18} \right\} - \left\{ \frac{\zeta_c}{\bar{K}\Gamma} - \frac{\pi\mu_c}{3} \right\} \frac{\lambda}{64} \left\{ 2\ln \left| \frac{r_{12}}{\varsigma} \right| - \frac{1}{2} \right\} \right. \\ & \left. - \left\{ \frac{\zeta}{\Gamma} - \frac{\pi\bar{K}\mu}{3} \right\} \frac{1}{48} \left( \frac{\lambda}{12\bar{K}} \right)^2 \left\{ 8\ln \left| \frac{r_{12}}{\varsigma} \right|^2 + 4 \left| \frac{r_{12}}{\varsigma} \right| - 1 \right\} \right] \frac{1}{r_{12}} \quad (\text{I.H.10}) \end{aligned}$$

where  $\dot{r}_1^{\parallel} = \dot{\mathbf{r}}_1 \cdot \hat{\mathbf{r}}_{12}$ , with  $\mathbf{r}_1$  being the velocity of the  $-1/6$  defect 1 and  $\hat{\mathbf{r}}_{12}$  is the unit vector from the  $-1/6$  defect 2 to the  $-1/6$  defect 1, and  $r_{12}$  is the the separation between the two defects. Notice, that even to zeroth order in  $\lambda$ , this interaction is not purely repulsive – as pointed out earlier, a  $-1/6$  defect essentially acts like a sink for active fluid flow for  $\zeta > 0$  and this flow advects other defects, irrespective of their sign towards it. It is possible, if this flow is strong enough, for the interaction between two  $-1/6$  defects to be attractive not only at large scales, due to  $\lambda$ , but also at short scales. In contrast, the velocity of a  $+1/6$  defect due to another  $+1/6$  defect along the line joining it is

$$\begin{aligned} \dot{r}_1^{\parallel} = & \left[ \left\{ \frac{\zeta}{6\Gamma} + \frac{\pi\bar{K}\mu}{18} \right\} - \left\{ \frac{\zeta_c}{\bar{K}\Gamma} + \frac{\pi\mu_c}{3} \right\} \frac{\lambda}{64} \left\{ 2\ln \left| \frac{r_{12}}{\varsigma} \right| - \frac{1}{2} \right\} \right. \\ & \left. - \left\{ \frac{\zeta}{\Gamma} + \frac{\pi\bar{K}\mu}{3} \right\} \frac{1}{48} \left( \frac{\lambda}{12\bar{K}} \right)^2 \left\{ 8\ln \left| \frac{r_{12}}{\varsigma} \right|^2 + 4 \left| \frac{r_{12}}{\varsigma} \right| - 1 \right\} \right] \frac{1}{r_{12}} \quad (\text{I.H.11}) \end{aligned}$$

where, again,  $\dot{r}_1^{\parallel} = \dot{\mathbf{r}}_1 \cdot \hat{\mathbf{r}}_{12}$ , with  $\mathbf{r}_1$  now being the velocity of the  $+1/6$  defect 1 and  $\hat{\mathbf{r}}_{12}$  being the unit vector from the  $+1/6$  defect 2 to the  $+1/6$  defect 1, and  $r_{12}$  is the the separation between the two defects. Thus, the two-particle interactions between defects are non-mutual and depends on the sign of both the defects. The many-body physics of a collection of  $\pm 1/6$  defects is therefore likely to be unlike theories of equilibrium defects. It is possible that such interactions may lead to charge-separation. However, we leave an examination of the many-body physics of defects and the defect-unbinding transition for future work.

### I. Hexatics with disclinations

In this section we will write down the hydrodynamic equations for a hexatic with a finite density of free disclinations (i.e. above the disclination-unbinding transition). Following [25] now define

$$\nabla\theta = \mathbf{v}_h \quad (\text{I.I.1})$$

in analogy with the superfluid velocity field. We define a disclination density by

$$\nabla \times \mathbf{v}_h = S \quad (\text{I.I.2})$$

where

$$S = 2\pi \sum_i s_i \delta(\mathbf{r} - \mathbf{r}_i) \quad (\text{I.I.3})$$

We also define a disclination current

$$\mathbf{J}_6 = 2\pi \sum_i s_i \dot{\mathbf{r}}_i \delta(\mathbf{r} - \mathbf{r}_i) \quad (\text{I.I.4})$$

This implies

$$\nabla \times (\partial_t \mathbf{v}_h - \boldsymbol{\epsilon} \cdot \mathbf{J}_6) = 0 \quad (\text{I.I.5})$$

Using the equation of motion for  $\theta$  in the absence of free disclinations for the irrotational part of the  $\mathbf{v}_h$  dynamics, we then obtain

$$\partial_t \mathbf{v}_h = \boldsymbol{\epsilon} \cdot \mathbf{J}_6 + \frac{1}{2} \nabla(\epsilon_{ij} \partial_i v_j) + \Gamma_6 K \nabla(\nabla \cdot \mathbf{v}_h) \quad (\text{I.I.6})$$

The other two dynamical equations remain unchanged:

$$\partial_t \rho = -\nabla \cdot \mathbf{g} = -\nabla \cdot (\rho \mathbf{v}). \quad (\text{I.I.7})$$

$$\rho \partial_t \mathbf{v} = -\frac{K}{2} (\hat{z} \times \nabla) \nabla(\nabla \cdot \mathbf{v}_h) - \rho \nabla \frac{\delta F}{\delta \rho} - \zeta \hat{z} \times \mathbf{v}_h - \zeta_c \hat{z} \times (\hat{z} \times \mathbf{v}_h) - \Gamma \mathbf{v} + \Gamma_c \hat{z} \times \mathbf{v} \quad (\text{I.I.8})$$

To compute  $\mathbf{J}_6$ , we write down the Fokker-Planck equation implied by (I.H.3). Note that that equation corresponds to *free* defects. The bound defects will be taken into account by a bound dielectric constant  $\epsilon_c$  as in [25]. We rewrite (I.H.3) as

$$\dot{\mathbf{r}}_i = \frac{1}{\Gamma} [\zeta \boldsymbol{\epsilon} \cdot \mathbf{v}_h|_{\mathbf{r}=\mathbf{r}_i} + \zeta_c \mathbf{v}_h|_{\mathbf{r}=\mathbf{r}_i}] + 2\pi s_i K (\mu \boldsymbol{\epsilon} \cdot \mathbf{v}_h|_{\mathbf{r}=\mathbf{r}_i} + \mu_c \mathbf{v}_h|_{\mathbf{r}=\mathbf{r}_i}) + \boldsymbol{\chi} \quad (\text{I.I.9})$$

which yields the current

$$\mathbf{J}_{6\text{free}} = \frac{1}{\Gamma} [\zeta \boldsymbol{\epsilon} \cdot \mathbf{v}_h + \zeta_c \mathbf{v}_h] S_{\text{free}} + \left[ \frac{\pi}{3} K (\mu \boldsymbol{\epsilon} \cdot \mathbf{v}_h + \mu_c \mathbf{v}_h) \right] n_f - \mu T \nabla S_{\text{free}} \quad (\text{I.I.10})$$

Here,  $n_f$  is the density of free disclinations. For dynamics near the transition, we take the bound charges into account by the use of a dielectric constant  $\epsilon_c$  which yields

$$\epsilon_c \nabla \times \mathbf{v}_h = S_{\text{free}} \quad (\text{I.I.11})$$

$$\epsilon_c \partial_t \mathbf{v}_h = \boldsymbol{\epsilon} \cdot \mathbf{J}_{6\text{free}} + \frac{1}{2} \nabla(\epsilon_{ij} \partial_i v_j) + \Gamma_6 K \nabla(\nabla \cdot \mathbf{v}_h). \quad (\text{I.I.12})$$

while the other equations remain the same. This equation together with the definition (I.I.10), clearly demonstrates that, for a finite  $n_f$ ,  $\mathbf{v}_h$  at long times relaxes to a value governed by  $\nabla(\epsilon_{ij} \partial_i v_j)$ . Therefore, the active terms in (I.I.8) with the coefficients  $\zeta$  and  $\zeta_c$  simply lead to the usual and odd viscosities [5]. This implies that disclination-unbinding in active chiral hexatics results in an active chiral isotropic fluid whose dynamics was discussed in detail in [5].



## J. Implications for chiral nematics

We now discuss how the physics we uncovered in this paper affects the possible existence of order in chiral nematics. First, nonlinearities of  $\sim (\nabla\theta)^2$  that we discussed is also present in chiral nematics, both on substrates and suspensions in an incompressible fluid. However, this doesn't modify the prediction of long-range order of chiral nematic suspensions in momentum conserved incompressible fluids discussed in [7] since there the fluctuations of the angle field are much smaller *even within the linear theory*. Therefore, let us consider chiral nematic on a substrate. For a non-rotating chiral nematic oriented along  $\hat{x}$ , uniaxial asymmetry implies that the chiral nonlinearity is not simply  $\sim (\nabla\theta)^2$  but  $\lambda_1(\partial_x\theta)^2 + \lambda_2(\partial_y\theta)^2$ . The chiral quadratic nonlinearities in nematics have the form  $\lambda_1(\partial_x\theta)^2 + \lambda_2(\partial_y\theta)^2$  where  $\lambda_1$  and  $\lambda_2$  are independent coefficients and  $y$  is the coordinate transverse to the ordering direction (this is in addition to the nonlinearities present even in achiral nematics which have the form  $\partial_x\theta\partial_y\theta$  and  $\theta\partial_x\partial_y\theta$ ). For  $\lambda_1/\lambda_2 < 0$  these nonlinearities are *irrelevant* [18–20, 35]. This would seem to suggest that in this case the chiral nematic must have QLRO since the achiral nonlinearities are always irrelevant in the nematic state [21], and their coefficients go to 0 at large scales. However, this is probably not the case. The reason that the *achiral* nonlinearities are irrelevant in a nematic is that they are *anisotropic* and the anisotropy of the nematic state is destroyed at large scale since the phase only has QLRO [22]. But this should *also* imply that at large scales  $\lambda_1/\lambda_2$  should flow to 1 *irrespective* of their initial values. In other words,  $\lambda_1 - \lambda_2$  must go to 0 as a typically small power of the wavevector (this power is the nonuniversal exponent controlling the asymptotic decay of the nematic order parameter). This should imply that at large scales the chiral nonlinearity *even* in a nematic *must* be  $\propto (\nabla\theta)^2$ . But we have already established that this nonlinearity is *relevant* and destroys QLRO. Thus, we expect that even chiral nematic on substrates will display only short-range order. We also point out that the effect of non-mutual interactions between defects have not been examined for chiral nematics as well as achiral nematics. Such interactions may fundamentally modify the physics of defect unbinding and we will consider this in a future publication.

## II. CHIRAL ACTIVE SOLIDS

### A. Active chiral solids on a substrate

Starting from the hexatic phase, when the density of active particles is increased or the noise strength is decreased beyond a critical value there is a phase transition to the solid phase which breaks translational symmetry in addition to the rotation symmetry. In this section, we therefore write down the theory of a chiral hexatic solid on a substrate generalising the work of [6]. In the next sections we will demonstrate that unbinding of dislocations in a chiral active solid yields a chiral active hexatic.

A solid is characterised by a spatially periodic mass-density wave; deviations away from a reference configuration of this mass density wave, characterised by the displacement field  $\mathbf{u}$  are the Goldstone mode of broken translation symmetry and are therefore hydrodynamic. Since a uniform  $\mathbf{u}$  just implies a global translation of the solid as a whole, all physical quantities such as forces must be due to spatial variations of  $\mathbf{u}$ . We therefore define the linearised antisymmetric and symmetric displacement gradient tensors of  $\mathbf{u}$ :

$$W_{ij}^a = \frac{1}{2}(w_{ij} - w_{ji}) \quad (\text{II.A.1})$$

$$W_{ij}^s = \frac{1}{2}(w_{ij} + w_{ji}) \quad (\text{II.A.2})$$

where  $w_{ij} = \partial_i u_j$  is the displacement gradient tensor. In what follows, we will also use the trace removed part of the symmetric displacement gradient tensor:

$$W_{ij} = \frac{1}{2}(w_{ij} + w_{ji} - \nabla \cdot \mathbf{u} \delta_{ij}) \quad (\text{II.A.3})$$

While the rotation symmetry remains broken in the crystalline phase, deviations from the orientationally ordered phase characterised by  $\theta$  are no longer soft (i.e. hydrodynamic) in the solid phase since a pure rotation also affects the displacement field (technically, this means that the static structure factor of angular fluctuations does not diverge at small  $q$ ,  $\lim_{q \rightarrow 0} \langle |\theta|^2 \rangle \rightarrow \text{const.}$  and their relaxation rate as  $q \rightarrow 0$  remains finite – a consequence of Anderson-Higgs mechanism [13, 14]). Instead,  $\theta$  is slaved to the antisymmetric part of the displacement gradient tensor which describes a rigid rotation of the mass-density wave:

$$F_\theta = \int \frac{A}{2} \left[ \theta - \frac{1}{2} \nabla \times \mathbf{u} \right]^2 + \frac{K}{2} (\nabla\theta)^2. \quad (\text{II.A.4})$$

Further, since the global rotation of the solid is a symmetry, there can be no other free energy term involving  $W_{ij}^a$  at the harmonic order.

We now build the equations of motion of chiral active crystals in terms of the mass density  $\rho$ , the displacement field  $\mathbf{u}$  (we will eliminate terms involving  $\theta$  in favour of  $\mathbf{W}^a$  using (II.A.4):  $\epsilon_{ij}\theta = W_{ij}^a = 1/2(\partial_i u_j - \partial_j u_i)$ ) and the velocity field  $\mathbf{v}$ . In a perfect crystal, without any vacancy or interstitial, the motion of a density wave, characterised by  $\partial_t \mathbf{u}$ , must exactly correspond to mass motion i.e.,  $\partial_t \mathbf{u} = \mathbf{v}$ . In this case, the density is slaved to dilations of the crystal via

$$\partial_t(\rho + \rho_0 \nabla \cdot \mathbf{u}) = 0 \quad (\text{II.A.5})$$

and, thus, the dynamics of the density field need not be separately considered. However, the presence of vacancies and interstitials spoil the correspondence between mass and structural motion. We first discuss the hydrodynamics of perfect crystals and next the more general case with a finite density of vacancies and interstitials.

### 1. Perfect crystals: No vacancies or interstitials

In this case, the density field does not matter, the time-derivative of the displacement field is simply the velocity field and the hydrodynamic theory only consists of the force balance equation for a crystal on a substrate:

$$\begin{aligned} \rho_0 \partial_t \mathbf{v} &= \rho_0 \partial_t^2 \mathbf{u} = \nabla \cdot \left[ \mu_s \mathbf{W} + \frac{1}{2} \mu_b (\nabla \cdot \mathbf{u}) \mathbf{I} + \zeta_{cs} \boldsymbol{\epsilon} \cdot \mathbf{W} + \frac{1}{2} \zeta_{cb} \boldsymbol{\epsilon} (\nabla \cdot \mathbf{u}) + \zeta \boldsymbol{\epsilon} \theta - \zeta_c \mathbf{I} \theta \right] - \Gamma \mathbf{v} - \Gamma_c \boldsymbol{\epsilon} \cdot \mathbf{v} \\ &= \nabla \cdot \left[ \mu_s \mathbf{W} + \frac{1}{2} \mu_b (\nabla \cdot \mathbf{u}) \mathbf{I} + \zeta \mathbf{W}^a + \zeta_{cs} \boldsymbol{\epsilon} \cdot \mathbf{W} + \frac{1}{2} \zeta_{cb} \boldsymbol{\epsilon} (\nabla \cdot \mathbf{u}) - \zeta_c \boldsymbol{\epsilon} \cdot \mathbf{W}^a \right] - \Gamma \partial_t \mathbf{u} - \Gamma_c \boldsymbol{\epsilon} \cdot \partial_t \mathbf{u}, \end{aligned} \quad (\text{II.A.6})$$

where the second line is explicitly written only in terms of  $\mathbf{u}$ . The terms in the square brackets in (II.A.6) constitute the elastic active stress while the remain two are dissipative frictions. The first two terms in the square brackets, with the coefficients  $\mu_s$  and  $\mu_b$  denote the standard shear and bulk response of a solid material. The third and fourth, with the coefficients  $\zeta_{cs}$  and  $\zeta_{cb}$  denote active chiral forces due to shear and bulk strains. These forces were first presented in [6] and their consequences were discussed in detail there. The term  $\zeta_{cs} \boldsymbol{\epsilon} \cdot \mathbf{W}$  is a symmetric tensor and therefore, this force is present even in momentum and angular momentum conserved active chiral solids (for a similar chiral force in active nematics, see [7]), while  $\zeta_{cb} \boldsymbol{\epsilon} (\nabla \cdot \mathbf{u})$  is a purely antisymmetric tensor, and therefore, it can only be present in systems that do not conserve angular momentum. The terms with the coefficients  $\zeta$  and  $\zeta_c$  are present in theory of hexatic as well, but in the solid phase can be re-expressed in terms of the antisymmetric displacement gradient tensor. Recall that  $\zeta$  is *achiral* but is only allowed in systems that do not conserve angular momentum while  $\zeta_c$  is chiral. The final two terms are the usual and the chiral friction. We now calculate the overdamped mode structure (ignoring inertia) implied by this equation:

$$\begin{aligned} \omega_{\pm} &= -\frac{iq^2}{4(\Gamma^2 + \Gamma_c^2)} \left[ \{ \Gamma(2\mu_s + \mu_b + \zeta) + \Gamma_c(2\zeta_{cs} - \zeta_{cb} + \zeta_c) \} \right. \\ &\quad \left. \pm \sqrt{\{ \Gamma(2\mu_s + \mu_b + \zeta) + \Gamma_c(2\zeta_{cs} - \zeta_{cb} + \zeta_c) \}^2 - 4\{(\mu_s + \mu_b)(\mu_s + \zeta) + (\zeta_{cs} - \zeta_{cb})(\zeta_{cs} + \zeta_c)\}(\Gamma^2 + \Gamma_c^2)} \right] \end{aligned} \quad (\text{II.A.7})$$

In equilibrium, the term in the square bracket is purely real for  $\mu_s, \mu_b > 0$  leading to a pair of diffusive modes (the usual transverse and longitudinal sounds modes of an underdamped spild are transformed into a pair of diffusive modes in the overdamped case). However, as discussed in [6], this need not be the case in chiral active solids. In this case, the term inside the square brackets may develop an imaginary part implying the existence of a propagating wave with dispersion  $\omega \sim q^2$  which is also damped at  $\mathcal{O}(q^2)$ . Chirality is essential for there to be a propagating part in the overdamped dispersion relation. However, chiral propagating wave may be present *even when* there is no displacement-dependent active force, i.e., the elastic forces are purely passive, but there is a chiral active friction. In this case, the frequency  $\omega_{\pm}$  develop a real (i.e. propagating) part when  $\Gamma_c^2 \mu_s (\mu_s + \mu_b) / \Gamma^2 \mu_b^2 > 1/4$ .

Though our theory of active chiral solids contain two extra forces in comparison to the theory presented in [6], the mode structure (II.A.7) is not qualitatively distinct from the one that would be obtained by ignoring  $\zeta$  and  $\zeta_c$  as was done in [6]. In fact,  $\zeta$  can be eliminated by the redefinition  $\mu_s \rightarrow \mu_s + \zeta$  and  $\mu_b \rightarrow \mu_b - \zeta$  and  $\zeta_c$  can be eliminated by the redefinition  $\mu_{cs} \rightarrow \mu_{cs} + \zeta_c$  and  $\mu_{cb} \rightarrow \mu_{cb} - \zeta_c$ . This is expected since  $\nabla \cdot \mathbf{W}^a = \nabla \cdot (\mathbf{W} - (1/2)(\nabla \cdot \mathbf{u}) \mathbf{I})$ . Nevertheless,  $\zeta$  and  $\zeta_c$  present extra control parameters that can be used to tune the values of other passive and active coefficients. To see what we mean consider, for the moment, an *achiral* but active solid. In this case,  $\Gamma_c, \zeta_c, \zeta_{cs}$  and  $\zeta_{cb}$  are 0 and the only effect of activity enters via the  $\zeta$  term. In passive systems, the longitudinal diffusivity

$\propto (\mu_b + \mu_s)$  is always larger than the transverse diffusivity  $\propto \mu_s$  for positive bulk and shear moduli. In an active achiral solid, the longitudinal diffusivity remains the same but the transverse diffusivity is  $\propto \mu_s + \zeta$  and can thus be larger than the longitudinal diffusivity. Thus, in this case, a large active force can make the effective bulk modulus negative.

## 2. Crystals with vacancies and interstitials

As discussed earlier, if vacancies and interstitials are present, the density field is no longer slaved to dilations and the motion of the phase field of the crystal,  $\dot{\mathbf{u}}$  is not slaved to the mass motion and is no longer the centre-of-mass velocity. Following [25] we now define a net conserved (signed) density of vacancies and interstitials:

$$\delta N = \delta \rho + \rho_0 \nabla \cdot \mathbf{u}, \quad \partial_t \delta N = -\nabla \cdot \mathbf{J} \quad (\text{II.A.8})$$

where  $\mathbf{J}$  is the current associated with vacancy density. The displacement field equation becomes

$$\partial_t \mathbf{u} = \mathbf{v} - \frac{1}{\rho_0} \mathbf{J} \quad (\text{II.A.9})$$

We now construct a constitutive equation for the vacancy current  $\mathbf{J}$  based on symmetry arguments:

$$\mathbf{J} = -\Gamma_N \rho_0 \left[ \nabla \left( \chi^{-1} \frac{\delta N}{\rho_0} + \beta \nabla \cdot \mathbf{u} + \beta_c \boldsymbol{\epsilon} : (\nabla \mathbf{u}) \right) + \beta_s \nabla \cdot \mathbf{W} + \beta_{sc} \nabla \cdot (\boldsymbol{\epsilon} \cdot \mathbf{W}) + \beta_a \nabla \cdot \mathbf{W}^a + \beta_{bc} \boldsymbol{\epsilon} \cdot \nabla (\nabla \cdot \mathbf{u}) \right]. \quad (\text{II.A.10})$$

The first two terms  $\propto \nabla(\chi^{-1} \delta N / \rho_0 + \beta \nabla \cdot \mathbf{u})$  arise in standard theories of solid hydrodynamics [25] and denote the gradient of the effective chemical potential for vacancies and interstitials. The term  $\beta_s \nabla \cdot \mathbf{W}$  can arise in equilibrium systems as well. The four remaining terms are not allowed in passive systems (though, as discussed in the last section, the terms with the coefficients  $\beta_c$  and  $\beta_a$  can be absorbed by suitable redefinitions of  $\beta$  and  $\beta_s$  and  $\beta_{sc}$  and  $\beta_{bc}$  respectively) and have the same form as the various active forces in (II.A.6). The terms with coefficients  $\beta_a$  and  $\beta_{bc}$  are solenoidal and therefore, does not affect the dynamics of  $\delta N$ . They do, however, affect the dynamics of the displacement field. The momentum density equation is only marginally modified from (II.A.6) and becomes

$$\rho_0 \partial_t \mathbf{v} = -\beta_2 \nabla \frac{\delta N}{\rho_0} + \nabla \cdot \left[ \mu_s \mathbf{W} + \frac{1}{2} \mu_b (\nabla \cdot \mathbf{u}) \mathbf{I} + \zeta \mathbf{W}^a + \zeta_{cs} \boldsymbol{\epsilon} \cdot \mathbf{W} + \frac{1}{2} \zeta_{cb} \boldsymbol{\epsilon} (\nabla \cdot \mathbf{u}) - \zeta_c \boldsymbol{\epsilon} \cdot \mathbf{W}^a \right] - \Gamma \mathbf{v} - \Gamma_c \boldsymbol{\epsilon} \cdot \mathbf{v}, \quad (\text{II.A.11})$$

In equilibrium,  $\beta_2$  had to be equal to  $\beta$ , since they had to originate from the same free-energy term coupling the vacancy density and the dilation  $\propto \delta N \nabla \cdot \mathbf{u}$  but that is not necessary in the nonequilibrium context under consideration. This constitutes a complete and general description of the hydrodynamic theory of chiral active solids which goes beyond the one considered by [6].

## B. Theory of dislocation unbinding in chiral active solids – connection to chiral active hexatics

A two-dimensional passive solid undergoes a dislocation unbinding transition to a hexatic phase upon increasing the noise (or decreasing density). In this section, we consider a phenomenological theory of a dislocation unbinding transition in a *chiral active* solid on a substrate and demonstrate that the chiral hexatic phase discussed earlier emerges from this, at least in a finite system (for large enough system sizes the hexatic phase itself is destroyed). In the solid phase, without any dislocation, the displacement field  $\mathbf{u}$  is single-valued everywhere. However, this is no longer the case in the presence of a dislocation;  $\mathbf{u}$  cannot be single-valued at the location of dislocations. This implies,

$$\epsilon_{ki} \partial_k w_{ij} = a_0 B_j \quad (\text{II.B.1})$$

where  $a_0$  is a length-scale, typically the lattice spacing,  $w_{ij}$  is the displacement gradient tensor as earlier and  $\mathbf{B}$  is the Burger's vector charge density

$$\mathbf{B} = \sum_{\alpha} \mathbf{b}^{\alpha} \delta(\mathbf{r} - \mathbf{R}^{\alpha}). \quad (\text{II.B.2})$$

Here,  $\mathbf{b}^{\alpha}$  is the Burger's vector of a dislocation at the point  $\mathbf{R}^{\alpha}$ . Topological charge conservation implies that the Burger's vector density is constant, and

$$\partial_t \mathbf{B} = -\nabla \cdot \mathbf{J}^B; \quad J_{ij}^B = \sum_{\alpha} \mathbf{b}_i^{\alpha} \dot{R}_j^{\alpha} \delta(\mathbf{r} - \mathbf{R}^{\alpha}) \quad (\text{II.B.3})$$

This together with (II.B.1) and (II.A.9) implies that

$$\partial_t w_{ij} = a_0 \epsilon_{ik} J_{jk}^B + \partial_i v_j - \frac{1}{\rho_0} \partial_i J_j. \quad (\text{II.B.4})$$

The equation of motion for the signed vacancies and interstitials (II.A.8) also gets modified due to the presence of dislocations

$$\partial_t \delta N = -\nabla \cdot \mathbf{J} + \rho_0 a_0 \epsilon_{ik} J_{ik}^B. \quad (\text{II.B.5})$$

with the motion of dislocations acting as sources and sinks of vacancies and interstitials [25]. In passive systems dislocations move due to the Peach-Koehler force [25, 30] which determines the dislocation current up to a phenomenological mobility tensor. In active systems an analogue of a Peach-Koehler force (i.e., the force on a dislocation) may be calculated, for instance, starting from a phase-field crystal model [26–28]. However, this is technically extremely complicated. Instead, in the spirit of phenomenological theories, we construct an expression for  $\mathbf{J}^B$  directly in the phase in which there is an *average* dislocation density  $n_f$  (i.e., above the dislocation unbinding transition) and demonstrate that this corresponds to the hexatic state. Dislocations must move due to smooth gradients of the displacement field and therefore,  $J_{ij}^B$  must depend on  $w_{ij}$ . However, it *cannot* depend on the *anti*-symmetric part of  $w_{ij}$  i.e., on  $\mathbf{W}^a$  since a constant  $\mathbf{W}^a$  describes a rigid rotation and such a rigid rotation should not lead to a current. Therefore,  $\mathbf{J}_{ij}^B$  can only depend on the symmetric part of  $w_{ij}$  and  $\delta N$

$$J_{ij}^B = n_f a_0 [\lambda_{c1} W_{ij} + \lambda_1 \epsilon_{ik} W_{kj} + \lambda_{c2} \delta_{ij} \nabla \cdot \mathbf{u} + \lambda_2 \epsilon_{ij} \nabla \cdot \mathbf{u} + \lambda_{c3} \delta_{ij} \delta N + \lambda_3 \epsilon_{ij} \delta N] + T \partial_j B_i. \quad (\text{II.B.6})$$

where  $\lambda_1, \lambda_2, \lambda_3, \lambda_{c1}, \lambda_{c2}$  and  $\lambda_{c3}$  are phenomenological coefficients. The final term is a diffusive piece of the current proportional to the gradient of dislocation density. Now, using the definitions  $W_{ij}^a = \epsilon_{ij} \theta$  and  $\delta N = \delta \rho + \rho_0 \nabla \cdot \mathbf{u}$ , and (II.B.4), we obtain an equation for the  $\theta$  dynamics:

$$\partial_t \theta = \frac{a_0}{2} J_{ii}^B + \frac{1}{2} \epsilon_{ij} \partial_i v_j - \frac{1}{2\rho_0} \epsilon_{ij} \partial_i J_j = a_0^2 n_f [\lambda_{c3} \delta \rho + (\lambda_{c2} + \lambda_{c3} \rho_0) \nabla \cdot \mathbf{u}] + \frac{1}{2} \epsilon_{ij} \partial_i v_j - \frac{1}{2\rho_0} \epsilon_{ij} \partial_i J_j \quad (\text{II.B.7})$$

and for  $\nabla \cdot \mathbf{u}$

$$\partial_t \nabla \cdot \mathbf{u} = a_0 \epsilon_{ik} J_{ik}^B + \nabla \cdot \mathbf{v} - \frac{1}{\rho_0} \nabla \cdot \mathbf{J} = 2a_0^2 n_f [\lambda_3 \delta \rho + (\lambda_2 + \lambda_3 \rho_0) \nabla \cdot \mathbf{u}] + \nabla \cdot \mathbf{v} - \frac{1}{\rho_0} \nabla \cdot \mathbf{J} \quad (\text{II.B.8})$$

In the high temperature phase,  $n_f$  is large (i.e., there is a high density of free dislocations) and we can write

$$\nabla \cdot \mathbf{u} = -\frac{\lambda_3}{(\lambda_2 + \lambda_3 \rho_0)} \delta \rho - \frac{1}{2a_0^2 n_f (\lambda_2 + \lambda_3 \rho_0)} \nabla \cdot \mathbf{v} + \dots \quad (\text{II.B.9})$$

Using this in the equation for  $\partial_t \theta$ , we obtain

$$\partial_t \theta = a_0^2 n_f \left[ \frac{\lambda_{c3} \lambda_2 - \lambda_3 \lambda_{c2}}{(\lambda_2 + \lambda_3 \rho_0)} \right] \delta \rho - \frac{(\lambda_{c2} + \lambda_{c3} \rho_0)}{2(\lambda_2 + \lambda_3 \rho_0)} \nabla \cdot \mathbf{v} + \frac{1}{2} \epsilon_{ij} \partial_i v_j \dots \quad (\text{II.B.10})$$

where the ellipsis denotes terms at higher order order in gradients which lead, in particular to terms  $\sim \nabla^2 \theta$  [34]. This leads to an expression for the coupling  $\gamma_c$  of the hexatic phase (see (I.A.2)) in terms of the parameters of the dislocation current:

$$\gamma_c = -\frac{(\lambda_{c2} + \lambda_{c3} \rho_0)}{2(\lambda_2 + \lambda_3 \rho_0)} \quad (\text{II.B.11})$$

leads to the identification of  $\Omega_1$  in (I.D.1)

$$\Omega_1 = a_0^2 n_f \left[ \frac{\lambda_{c3} \lambda_2 - \lambda_3 \lambda_{c2}}{(\lambda_2 + \lambda_3 \rho_0)} \right] \quad (\text{II.B.12})$$

The density-dependent rotation rate  $\Omega_1$  is necessarily active; in a passive system the dislocation current must be obtained from a free-energy derivative implying that even in *chiral* systems it can only have the form

$$J_{ij}^B \sim \Gamma_1 (a_1 \delta N + a_2 \nabla \cdot \mathbf{u}) \epsilon_{ij} + \Gamma_2 (a_1 \delta N + a_2 \nabla \cdot \mathbf{u}) \delta_{ij} \quad (\text{II.B.13})$$

where  $a_1$  and  $a_2$  are arbitrary constants. Therefore, identifying  $\lambda_3 = \Gamma_1 a_1$ ,  $\lambda_{c3} = \Gamma_2 a_1$ ,  $\lambda_2 = \Gamma_1 a_2$ ,  $\lambda_{c2} = \Gamma_2 a_2$ , we find that  $\lambda_{c3}\lambda_2 = \Gamma_1\Gamma_2 a_1 a_2$  and  $\lambda_{c2}\lambda_3 = \Gamma_2\Gamma_1 a_1 a_2$ , and this term identically vanishes, as it should. We have not identified a term analogous to  $\Omega_0$  in sec. IB, i.e., a spontaneous rotation-rate at the steady-state density. Such a term would imply a constant term in the dislocation current density  $\propto \rho_0$ . This would imply a dislocation current *even* in a *perfectly* homogeneous active crystal. Such a dislocation current should imply the destruction of the solid phase *even* in the limit of zero noise due to dislocation-unbinding.

Finally, we consider the dynamics of the deviatoric part of the displament gradient tensor:  $W_{ij} = (w_{ij} + w_{ji} - w_{ii}\delta_{ij})/2$ ,

$$\partial_t W_{ij} = \frac{(\partial_i v_j + \partial_j v_i - \nabla \cdot \mathbf{v} \delta_{ij})}{2} + a_0 \frac{\epsilon_{ik} J_{jk}^B + \epsilon_{jk} J_{ik}^B - \epsilon_{ml} J_{ml}^B \delta_{ij}}{2}. \quad (\text{II.B.14})$$

This yields

$$\partial_t \mathbf{W} = \frac{(\nabla \mathbf{v} + (\nabla \mathbf{v})^T - \nabla \cdot \mathbf{v} \mathbf{I})}{2} - n_f a_0^2 [\lambda_1 \mathbf{I} - \lambda_{c1} \boldsymbol{\epsilon}] \cdot \mathbf{W} \quad (\text{II.B.15})$$

Thus, at high defect densities, when the L.H.S. of (II.B.15) can be ignored, the strain  $\mathbf{W}$  relaxes to

$$\mathbf{W} = \frac{1}{n_f a_0^2} [\lambda_1 \mathbf{I} - \lambda_{c1} \boldsymbol{\epsilon}]^{-1} \cdot \frac{(\nabla \mathbf{v} + (\nabla \mathbf{v})^T - \nabla \cdot \mathbf{v} \mathbf{I})}{2} \quad (\text{II.B.16})$$

This implies that the parts of the elastic stress tensor

$$\boldsymbol{\sigma} = \mu_s \mathbf{W} + \frac{1}{2} \mu_b (\nabla \cdot \mathbf{u}) \mathbf{I} + \zeta \mathbf{W}^a + \zeta_{cs} \boldsymbol{\epsilon} \cdot \mathbf{W} + \frac{1}{2} \zeta_{cb} \boldsymbol{\epsilon} (\nabla \cdot \mathbf{u}) - \zeta_c \boldsymbol{\epsilon} \cdot \mathbf{W}^a \quad (\text{II.B.17})$$

that are dependent on  $\mathbf{W}$  and  $\nabla \cdot \mathbf{u}$  yield bulk, shear and odd [5] viscosities in the active hexatic phase. The parts depending on  $\mathbf{W}^a$  however lead to the active forces in the hexatic (I.A.4), using the definition  $W_{ij}^a = \epsilon_{ij} \theta$ . This implies that the melting of the solid phase by dislocation unbinding leads to a active chiral hexatic.

---

\* nyomaitra07@gmail.com

- [1] S. Ramaswamy, Annu. Rev. Condens. Matter Phys., **1**, 323 (2010)
- [2] A. Maitra et al., Phys. Rev. Lett **124**, 028002 (2020)
- [3] S. R. De Groot, P. Mazur, Non-Equilibrium Thermodynamics, Dover Books on Physics (2011)
- [4] P. C. Martin, O. Parodi, P. S. Pershan, Phys. Rev. A **6**, 2401 (1972)
- [5] D. Banerjee et al, Nat. Comm. **8**, 1573 (2017)
- [6] C. Scheibner et al., Nat. Phys. (2020)
- [7] A. Maitra, M. Lenz, Nat. Commun. **10**, 920 (2019)
- [8] S. Tanida, K. Furuta, K. Nishikawa, T. Hiraiwa, H. Kojima, K. Oiwa, M. Sano, Phys. Rev. E **101**, 032607 (2020).
- [9] S. Shankar, S. Ramaswamy, M. C. Marchetti, Physical Review E **97**, 012707 (2018)
- [10] D. Forster, Hydrodynamic Fluctuations, Broken Symmetry, And Correlation Functions, Advanced Books Classics, Westview Press (1995)
- [11] D. R. Nelson, R. A. Pelcovits, Phys. Rev. B **16**, 2191 (1977)
- [12] D. Das, M. Barma, Phys. Rev. Lett. **85**, 1602 (2000)
- [13] P. W. Anderson, Phys. Rev. **130**, 439 (1963)
- [14] P. M. Chaikin, T. C. Lubensky, Principles of Condensed Matter Physics, Cambridge University Press (2000)
- [15] T. Markovich, E. Tjhung, M. E. Cates, New J. Phys. **21**, 112001 (2019)
- [16] A. Aubret et al., Nat. Phys. **14**, 1114 (2018)
- [17] A. Maitra, R. Voituriez, Phys. Rev. Lett **124**, 048003 (2020)
- [18] E. Altman et al., Phys. Rev. X **5**, 011017 (2015)
- [19] L. Chen, J. Toner, Phys. Rev. Lett. **111**, 088701 (2013)
- [20] D. E. Wolf, Phys. Rev. Lett. **67**, 1783 (1991).
- [21] S. Mishra, A. Simha, S. Ramaswamy, J. Stat. Mech. P02003 (2010)
- [22] D. R. Nelson, R. A. Pelcovits, Phys. Rev. B **16**, 2191 (1977)
- [23] L. P. Dadhichi, A. Maitra, S. Ramaswamy, arXiv: 1808.08997
- [24] S. Ramaswamy, J. Stat. Mech., 054002 (2017)
- [25] A. Zippelius, B. I. Halperin, D. R. Nelson, Phys. Rev. B **22**, 2514 (1980)
- [26] F. Alaïmo, S. Praetorius, A. Voigt, New J. Phys **18**, 083008 (2016)
- [27] A. M. Menzel, T. Ohta, H. Löwen, Phys. Rev. E **89**, 022301 (2014)

- [28] V. Heinonen et al., Phys. Rev. Lett. **116**, 024303 (2016)
- [29] L. M. Pismen, Phys. Rev. E **88**, 050502 (2013)
- [30] F. R. N. Nabarro, Theory of Crystal Dislocations, Dover Books on Physics and Chemistry (1987)
- [31] S. Shankar et al., Phys. Rev. Lett. **121**, 108002 (2018)
- [32] E. I. Kats, V. V. Lebedev, S. V. Malinin, JETP **95**, 714 (2002)
- [33] C. Denniston, Phys. Rev. B **54**, 6272 (1996)
- [34] M. C. Marchetti, K. Saunders, Phys. Rev. B **66**, 224113 (2002)
- [35] L. M. Sieberer, E. Altman, Phys. Rev. Lett. **121**, 085704 (2018)
- [36] G. Wachtel et al., Phys. Rev. B **94**, 104520 (2016)
